# Supplementary material for: Testing Firm Conduct
Source: arXiv:2301.06720 source file (2024-01-17)
Supplement: Supplementary file 2 [file AppendixBCScomparison.tex]

Flow:

* Comparison to the Optimal Instrument reasoning in BCS;

* We can think of BCS doing two conceptual steps:
1. Arguing that E[\Delta_1-\Delta_2\mid z] is the optimal instrument, discrete analogue of \cite{c87}
2. Obtain an approximation thereof with a flexible estimation method, RF
We construct in this way a "BCS Test" to analyze their procedure, subject to the caveats above.

* To facilitate the comparison between their procedure and standard RV testing as discussed in our paper, we will need to maintain some simplifications.
1. Suppose that, instead of RF, the approximation of the optimal instrument is implemented with a method that uses some linear function of an expanded set of the original exogenous variables; e.g., a linear sieve. While not same as RF, arguably this method can achieve similar flexibility; is similar to ANN (see work by Chen, Tamer), has "universal approximator" properties.
2. We suppose that the researcher uses the same sample to both fit the approximation of the optimal instruments and perform testing. This can be relaxed (?)

* Then, we can establish that:
1. The BCS test is degenerate in a strictly larger region than the RV test conducted with the same expanded set of instruments is;
2. In the absence of degeneracy in BCS, the asymptotic distribution of the BCS test is the same as that of an RV test conducted with the same expanded set of instrument that is used to construct the BCS optimal instruments;  hence, the power of the BCS test is no greater than the power of RV.

* Flexibility is an important component of the procedure, and deserves discussion
1. In population, flexibility can help reduce the space of degeneracy. Considering an expanded set of instruments allows to better approximate the conditional expectations E[\Delta_1-\Delta_0\mid z] and [\Delta_2-\Delta_0\mid z], so that there are cases where the RV test with just the original instruments is degenerate, but tests with larger set of instruments are not.
2. However, when considering inference, many instruments can create distortions in the asymptotic distribution of the test, causing size issues.
3. These issues could be addressed by sample splitting, so that a flexible implementation of RV is possible.

[Q: isn't THIS the optimal instrument?]
