# Supplementary material for: Testing Firm Conduct
Source: arXiv:2301.06720 source file (2024-01-17)
Supplement: Supplementary file 3 [file Robustness.tex]

This appendix provides additional details and robustness exercises for our empirical application. We first discuss the candidate conduct models in more detail.

\noindent \textbf{Description of the Models of Conduct:} Following \cite{v07}, the markups in market $t$ for a model $m$ among those we consider can be written in the following form:
\[\boldsymbol{\Delta}_{mt}=\underbrace{-(\boldsymbol{\Omega}^r_{mt} \odot \boldsymbol{D}^r_t)^{-1} \boldsymbol{s}_t}_{\boldsymbol{\Delta}^\text{downstream}_{mt}}\underbrace{-(\boldsymbol{\Omega}^w_{mt} \odot \boldsymbol{D}^w_t )^{-1} \boldsymbol{s}_t}_{\boldsymbol{\Delta}^\text{upstream}_{mt}}\]
where $\boldsymbol{\Omega}^r_{mt}$ and $\boldsymbol{\Omega}^w_{mt}$ are ownership matrices, $\boldsymbol{D}^w_t$ is the jacobian of retail share $\boldsymbol{s}_t$ with respect to wholesale price, and $\boldsymbol{D}^r_t$ is the jacobian of retail share with respect to retail price. The markup $\boldsymbol{\Delta}_{mt}$ implied by each model is the sum of downstream markups $\boldsymbol{\Delta}^\text{downstream}_{mt}$ and upstream markups $\boldsymbol{\Delta}^\text{upstream}_{mt}$. We can derive each model by using different assumptions on the ownership matrices:
\begin{enumerate}
    \item \textit{Zero wholesale margin}: Set $\boldsymbol{\Omega}^w_{mt}$ to a matrix of zeros, set $\boldsymbol{\Omega}^r_{mt}$ to a matrix of ones.
    \item \textit{Zero retail margin}: Set $\boldsymbol{\Omega}^w_{mt}$ to a matrix of zeros, and set $\boldsymbol{\Omega}^r_{mt}$ to a matrix  with element $(i,j)$ that is equal to one if products $i$ and $j$ are produced by the same manufacturer, and to zero otherwise. 
    \item \textit{Linear pricing}: Set $\boldsymbol{\Omega}^r_{mt}$ to a matrix of ones, and set $\boldsymbol{\Omega}^w_{mt}$ to a matrix  with element $(i,j)$ that is equal to one if products $i$ and $j$ are produced by the same manufacturer, and to zero otherwise. 
    \item \textit{Hybrid model}: Set $\boldsymbol{\Omega}^r_{mt}$ to a matrix of ones, and set $\boldsymbol{\Omega}^w_{mt}$ to a matrix  with element $(i,j)$ that is equal to one if products $i$ and $j$ are produced by the same manufacturer and $i$ is not a private label, and to zero otherwise. 
    \item \textit{Wholesale Collusion}: Set $\boldsymbol{\Omega}^r_{mt}$ and $\boldsymbol{\Omega}^w_{mt}$ to matrices of ones. \looseness=-1
    
\end{enumerate}

\noindent \textbf{Distributions of Predicted Markups:} To build intuition on the mechanics of the RV test, we report in Figure \ref{fig:Pmkups_plot} the distributions of predicted markups for the three sets of instruments that we use in the main text. All distributions are 
\begin{figure}[H] 
\centering \caption{Distributions of Predicted Markups}
\label{fig:Pmkups_plot}
    \begin{subfigure}{.49\linewidth}
    \centering
    \includegraphics[scale=0.49]{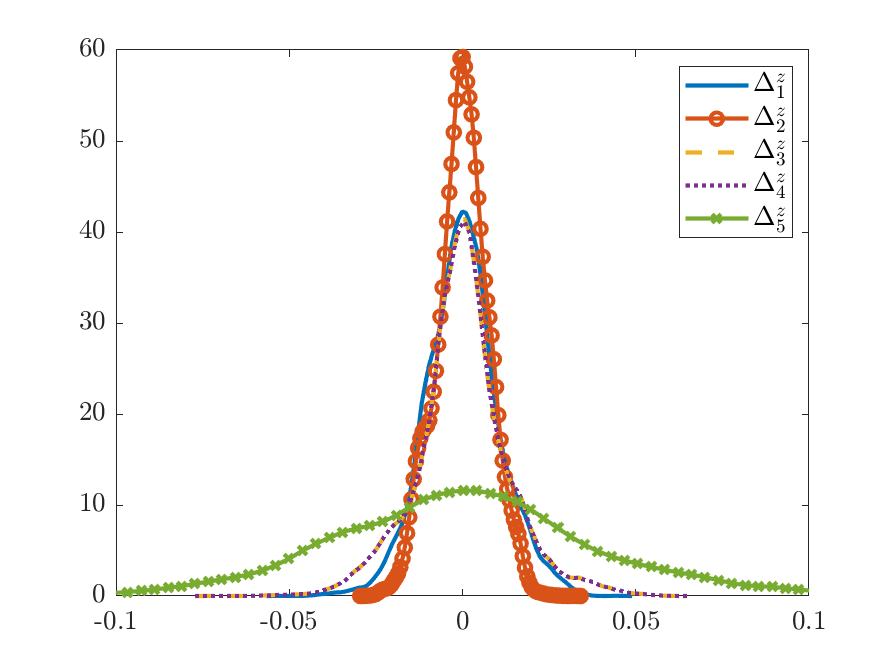}
    \caption{BLP95 IVs}
    \end{subfigure}
    \begin{subfigure}{.49\linewidth}
    \includegraphics[scale=0.49]{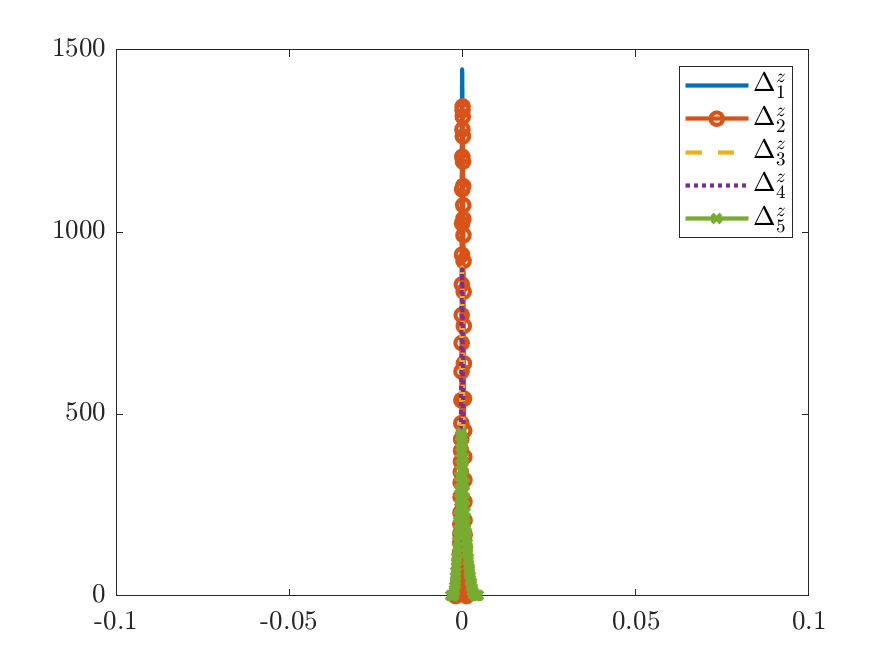}
    \caption{GH20 IVs}
    \end{subfigure}
    \begin{subfigure}{.49\linewidth}
    \includegraphics[scale=0.49]{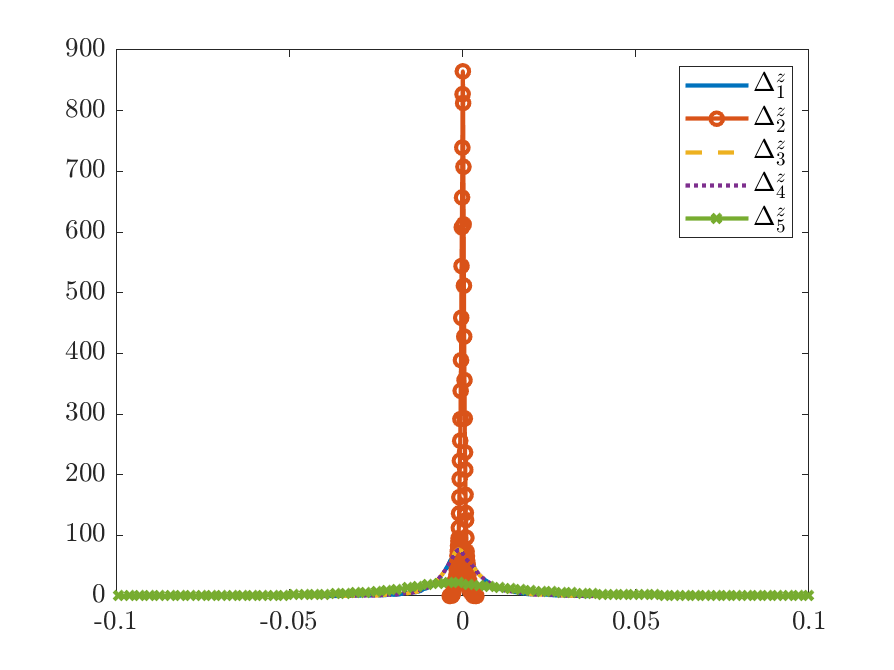}
    \caption{Rival Cost Shifters IVs}
    \end{subfigure}
    \caption*{\footnotesize{We report the distributions of $\Delta^z_{mi}$, the residualized predicted markups, for each model.}}
\vspace{-0.5cm}
\end{figure}     
\noindent centered at zero, since markups are residualized. The BLP95 instruments appear to generate meaningful differences in the distributions of predicted markups across models, thus making the test powerful. In contrast, the GH20 instruments generate distributions of predicted markups for the five models that are indistinguishable - the RV test has no power in this case. Finally, for the rival cost shifters instruments there is a clear distinction between the distribution of predicted markups for model 5 and all other distributions.  

While the figure helps interpretation, visual inspection of these distributions cannot substitute for formal RV testing, followed by the weak instruments diagnostic. In fact, interpreting the differences across distributions in terms of valid statistical statements requires the testing procedure we define.

\noindent \textbf{Alternative Sets of Instruments:} We perform RV testing using alternative sets of instruments. First, we combine the three sets of instruments that we use in the main text: BLP95, GH20 and rival cost shifters.\footnote{Results obtained using BLP95 and GH20 instruments together are similar.} We report in  Panel A of Table \ref{Tab:Instr_Rob} the effective $F$-statistics and MCS $p$-values for testing with these instruments. Combining the strong BLP95 instruments with the weak GH20 and rival cost shifters instruments lowers the effective $F$-statistics. In this case, while the instruments remain powerful and model 5 is firmly rejected, the MCS $p$-values for models 3 and 4 increase to 0.09 --- though still below the confidence level of 0.1 considered in \cite{hln11} and thus consistent with the RV test conducted with BLP95 instruments.

\begin{table}[htb]
\footnotesize
\caption{$F_\rho$ and MCS for Alternative Instruments}
\label{Tab:Instr_Rob}
\centering
\begin{threeparttable}
\begin{widetable}{.98\columnwidth}{lrrrrc}
\toprule
\textbf{Panel A: BLP95 + GH20 + Rival Cost} & \multicolumn{4}{c}{$F_\rho$}& MCS $p$-values\\
\multicolumn{1}{l}{($d_z=8$)}&\multicolumn{1}{c}{2}& \multicolumn{1}{c}{3}& \multicolumn{1}{c}{4}& \multicolumn{1}{c}{5}& \\
\cmidrule(lr){2-6}
1. Zero wholesale margin&65.7&21.5&21.5&91.7&0.71 \\
2. Zero retail margin&&30.1&30.2&80.1&1.00 \\
3. Linear pricing&&&36.3&33.1&0.09 \\
4. Hybrid model&&&&33.0&0.09 \\
5. Wholesale collusion&&&&&0.00 \\
\midrule
\textbf{Panel B: Difference in Cost Shifters IVs} & \multicolumn{4}{c}{$F_\rho$}& MCS $p$-values\\
\multicolumn{1}{l}{($d_z=1$)}&\multicolumn{1}{c}{2}& \multicolumn{1}{c}{3}& \multicolumn{1}{c}{4}& \multicolumn{1}{c}{5}& \\
\cmidrule(lr){2-6}
1. Zero wholesale margin&12.1&3.8&3.8&4.8&0.72\\
2. Zero retail margin&&7.1&7.0&8.1&0.19\\
3. Linear pricing&&&1.8&2.8&0.72\\
4. Hybrid model&&&&2.8&0.70\\
5. Wholesale collusion&&&&&1.00\\
\midrule
\textbf{Panel C: BLP Constant IVs} & \multicolumn{4}{c}{$F_\rho$}& MCS $p$-values\\
\multicolumn{1}{l}{($d_z=2$)}&\multicolumn{1}{c}{2}& \multicolumn{1}{c}{3}& \multicolumn{1}{c}{4}& \multicolumn{1}{c}{5}& \\
\cmidrule(lr){2-6}
1. Zero wholesale margin&63.6&28.0&28.0&91.3&0.61\\
2. Zero retail margin&&37.8&37.9&78.5&1.00\\
3. Linear pricing&&&50.1&29.3&0.02\\
4. Hybrid model&&&&29.1&0.02\\
5. Wholesale collusion&&&&&0.00\\
\bottomrule
\end{widetable}

\begin{tablenotes}[flushleft]
    \footnotesize
    \item[]Each panel reports $F_\rho$ for the pair of models indicated by the row and column, and the MCS $p$-values for each row model. With MCS $p$-values below 0.05 a row model is rejected at a confidence level $\alpha=0.05$.  Values of $F_\rho$ and MCS standard errors account for two-step estimation error; see Appendix \ref{sect:TwoStep} for details.
\end{tablenotes}
\end{threeparttable}
\end{table}    

In  Panel B of Table \ref{Tab:Instr_Rob} we construct rival cost shifters instruments by taking the sum of squared differences between own and rival transportation cost. This different functional form also results in an instrument that is weak for size (at the $0.10$ target) and power (at the $0.50$ target), now for every combination of models. Testing based on this instrument is uninformative.

Panel C of Table \ref{Tab:Instr_Rob} helps to shed light on the source of power of the BLP95 instruments. In this panel we perform testing using as instruments only the number of other products produced by the firm, and the number of total products produced by rival firms. These instruments are powerful, and deliver identical results to the BLP95 instrument set. Hence, the number of products is a key dimension of variation in the data for testing conduct in this application. \looseness=-1
