# Supplementary material for: Testing Firm Conduct
Source: arXiv:2301.06720 source file (2024-01-17)
Supplement: Supplementary file 6 [file Emipirical.tex]

\subsection{Data}\label{sec:data}

Our main source of data is the IRI Academic Dataset (see \cite{bkm08} for a description).  This dataset contains weekly price and quantity data for upcs sold in a sample of stores in the United States.  While this is the same data source as in \cite{v07}, it is not the same dataset as it covers a later time period and significantly more geographic markets.  Thus, our aim is not to replicate her findings; instead we seek to use this important empirical setting to illustrate our approach to testing. In cleaning the data, we try to mimic her choices as closely as possible.

Our data is for the year of 2010.\footnote{We choose to use only one year because the IRI dataset does not provide cross-reference for supermarket chains' identity across years and for computational reasons.} We define a market as a retail store-quarter.  We drop data coming from two geographic markets (``EAU CLAIRE'' and ``PITTSFIELD'') for which IRI does not provide geographical location information. We approximate the market size with a measure of the traffic in each store,  derived from the store-level revenue information from IRI. For approximately 5\% of stores, this approximation is poor resulting in an outside share below 50\%.  We drop these from our sample.  

In defining a product, we restrict attention to upcs labelled as ``yogurt'' in the IRI data and focus on the most commonly purchased sizes: 6, 16, 24 and 32oz.\footnote{For example, we drop products labelled ``soy yogurt'' and ``goat yogurt''}  Similar to \cite{v07}, we define a product as a brand-fat content-flavor-size, where flavor takes the value ``Plain'' or ``Other'' and fat content is either light (less than 4.5\% fat content) or whole.\footnote{Given that we lack detailed information for private label products,  we do not add other nutritional information.}  We further standardize package sizes to 6oz serving sizes.

Based on market shares, we exclude niche firms and products from the analysis. In particular, any firm which have less than a 5\% inside share  in all markets is dropped. We also drop products from a market which have an inside share lower than 0.1\% in that market and for which their cumulative inside share is not bigger than 1\%. After cleaning, our dataset has  205,123 observations for 5,034 markets corresponding to  1,309 stores.

We supplement our main dataset with county level demographics obtained from the Census Bureau's PUMS database which we match to the DMAs in the IRI data.  In particular, we draw 1000 households and record household income and age of the head of the household. We exclude households with income lower than \$12k or bigger than \$1 million. The demographic variables are adjusted to reflect their deviation from the mean.

We also measure transportation costs from manufacturer to retailer using average fuel cost times distance.  To do so, we use data on average regional on-highway diesel prices in dollars per gallon by quarter from the US Energy Information Administration.\footnote{https://www.eia.gov/dnav/pet/pet\_pri\_gnd\_dcus\_nus\_w.htm} Manufacturer plant locations were collected by hand.\footnote{We thank Xinrong Zhu for generously sharing this data with us.}
 
 Table \ref{Tab:summarystats} contains summary statistics for the main variables of interest in the paper.  
\begin{table}[!h]\footnotesize\caption{Summary Statistics}\label{Tab:summarystats}\centering

% Table created by stargazer v.5.2.2 by Marek Hlavac, Harvard University. E-mail: hlavac at fas.harvard.edu
% Date and time: Fri, Mar 12, 2021 - 03:58:35 PM
\begin{tabular}{@{\extracolsep{5pt}}lccccccc} 
\\[-1.8ex]\hline 
\hline \\[-1.8ex] 
 & \multicolumn{1}{c}{Mean} & \multicolumn{1}{c}{St. Dev.} & \multicolumn{1}{c}{Median} & \multicolumn{1}{c}{Max} & \multicolumn{1}{c}{Min} & \multicolumn{1}{c}{Pctl(25)} & \multicolumn{1}{c}{Pctl(75)} \\ 
\hline \\[-1.8ex] 
price & 0.759 & 0.295 & 0.676 & 2.690 & 0.186 & 0.549 & 0.911 \\ 
sales & 1,461.252 & 3,199.272 & 503.000 & 104,492.000 & 2.000 & 213.333 & 1,301.000 \\ 
shares & 0.007 & 0.012 & 0.003 & 0.280 & 0.00001 & 0.001 & 0.007 \\ 
outside share & 0.710 & 0.111 & 0.708 & 0.995 & 0.318 & 0.631 & 0.788 \\ 
size & 17.815 & 10.574 & 16 & 32 & 6 & 6 & 32 \\ 
light & 0.925 & 0.263 & 1 & 1 & 0 & 1 & 1 \\ 
number flavors & 5.388 & 5.811 & 3 & 35 & 1 & 1 & 8 \\ 
%private label & 0.088 & 0.283 & 0 & 1 & 0 & 0 & 0 \\ 
%price reduction & 0.309 & 0.277 & 0.3 & 1 & 0 & 0 & 0.5 \\ 
distance to plant & 493.066 & 476.568 & 392.471 & 2,670.635 & 25.702 & 198.643 & 546.187 \\ 
freight cost & 211.932 & 242.070 & 164.3 & 1,466 & 0 & 51.9 & 270.8 \\ 
\hline \\[-1.8ex] 
\end{tabular} 

\end{table}    

\subsection{Demand Model, Identification, and Estimation}

\noindent \textbf{Demand Model:}
We begin by describing our model of demand which follows a standard framework from  \cite{blp95}, as in \cite{v07}.  Each consumer $i$ receives utility from purchasing product $j$ in market $t$ according to the following utility index:
\begin{align}\label{eq:utility}
    u_{ijt} = \beta_i x_j + \alpha_i p_{jt} + \xi_{t} + \xi_{s} + \xi_{b(j)} + \xi_{jt} + \epsilon_{ijt} 
\end{align}
where $x_j$ includes a set of product characteristics: package size and dummy variables for whether the yogurt is low fat and for whether it is plain flavored. We also include the log of the number of flavors offered in the market, following \cite{ar05}. $p_{jt}$ represents the price charged for product $j$ in market $t$.   
All specifications have fixed effects for quarter, store and brand producing product $j$, denoted $\xi_{t}$, $\xi_{s}$, and $\xi_{b(j)}$ respectively.  $\xi_{jt}$ and $\epsilon_{ijt}$ denotes unobservable shocks at the product-market and the individual product market level, respectively.  Finally, we allow consumer preferences for characteristics $\beta_i$ and price $\alpha_i$ to vary across individuals. As in \cite{v07}, we do so by interacting their mean with individual level demographics for income and age of the head of household so that
\begin{align}
    \alpha_i &= \bar\alpha + \tilde\alpha\times D_i\\
    \beta_i &= \bar\beta + \tilde\beta\times D_i
\end{align}    
where $\bar\alpha$ and $\bar\beta$ represent the mean taste across consumers and $D_i$ denotes demographics.

To close the model of demand, we make additional assumptions which are standard in the literature.  In particular, we normalize the utility consumer $i$ receives from consuming the outside option as $u_{i0t} = \epsilon_{i0t}$.  The idiosyncratic errors $\epsilon_{jt}$ and $\epsilon_{i0t}$ are assumed to be distributed i.i.d. Type I extreme value. Under the assumption that each consumer purchases one unit of the good that gives her the highest utility, including the outside good, the market share of product $j$ in market $t$ takes the following form:      
\begin{equation}\label{eq:shares}
s_{jt} = \int \frac{\exp({\beta_{i}x_{j}  + \alpha_i p_{jt} +\xi_{t} + \xi_{s} + \xi_{b(j)}  + \xi_{jt}})}{1 +\sum_{l\in{\mathcal{J}_{t}}} \exp({\beta_{i}x_{l}  + \alpha_i p_{lt} +\xi_{t} + \xi_{s} + \xi_{b(l)}  + \xi_{lt}})}f(\alpha_i,\beta_i) \text{d}\alpha_i\text{d}\beta_i
\end{equation}

\noindent \textbf{Identification and Estimation:}   Demand estimation and testing can either be performed \textit{sequentially}, in which demand estimation is a preliminary step, or \textit{simultaneously} by stacking the demand and supply moments.  Following \cite{v07}, we adopt a sequential approach.  For the purposes of illustrating the empirical relevance of the findings in Sections 4 and 5, the computationally simpler simultaneous approach is sufficient.  We estimate demand following the approach developed in \cite{blp95}.  Including brand, store, and quarter fixed effects in (\ref{eq:utility}) controls for all unobservables that are constant either within a brand, a store, or a quarter. Thus, the source of endogeneity which threatens identification is limited to the set of unobservables that vary across these dimensions, denoted as $\xi_{jt}$.  
As prices and shares may be correlated with  $\xi_{jt}$, instruments are then required to identify the coefficient on price $\alpha_i$ and parameters for the individual specific components of utility, $\tilde\alpha$ and $\tilde\beta$, as these latter parameters enter the model non-linearly.    

We use a standard set of instruments.  For each brand in each market, we interact the average highway fuel cost for the region of the country where that market is located with the distance from the store to the brand's nearest manufacturing plant.  As we lack information on plant location for some products, including private labels, we interact the unobserved vector of fuel costs for all observations with a dummy indicating that plant location is observed.  This cost shifter provides exogenous variation to identify the coefficient on price, $\alpha$. 

The non-linear parameters are identified using instrumental variables proposed in \cite{gh19}.  For the nonlinear price parameters on demographics $\tilde\alpha$, we interact the fuel cost instrument with the mean of the demographics for the DMA in which the market is located. For $\tilde\beta$, we interact the observed characteristics with the mean of the demographics for the DMA in which the market is located.  Under the timing assumptions of the model, \cite{gh19} demonstrate that this interaction provides exogenous cross-sectional variation to identify the parameters of interest.  

Estimation proceeds via GMM.     For each guess of the non-linear parameters, we employ the contraction presented in \cite{blp95} to recover the mean utility of each product in each market.  We then regress the mean utilities on price and a set of dummy variables for the fixed effects via two-stage least squares and recover the unobserved product market unobservables as residuals.  We then interact these residuals with the instruments to form the sample moments which enter the GMM objective function. The GMM procedure recovers estimates of the nonlinear parameters, $\tilde\alpha$ and $\tilde\beta$, as well as the price coefficient, $\alpha$, and the fixed effects.  We compute demand estimates using the PyBLP package developed in \cite{cg19}.\footnote{We refer to PyBLP documentation website https://pyblp.readthedocs.io/en/stable/index.html# for detailed information of the methods used.}.

\noindent \textbf{Results:} Results for demand estimation are reported in Table \ref{Tab:demand}.  As a reference, we report estimates of a standard logit model of demand in Columns 1 and 2.  In Column 1, the logit model is estimated via OLS while in Column 2, we use fuel cost as an instrument for price and estimate the model via 2SLS.  We see a large reduction in the price coefficient, indicative of endogenity not controlled for by the fixed effects.  Columns 3 and 4 report estimates of the full demand model.  Our full demand model generates reasonable elasticities which are comparable to those obtained in \cite{v07} who finds a mean own price elasticity of -5.64.      

\begin{table}[H]\footnotesize
\caption{Demand Estimates}\centering
    \begin{widetable}{.98\columnwidth}{lrrrrrr}
\toprule
& \multicolumn{2}{c}{(1) Logit-OLS}  & \multicolumn{2}{c}{(2) Logit-2SLS}  & \multicolumn{2}{c}{(3) BLP}   \\
\cmidrule(lr){2-3} \cmidrule(lr){4-5} \cmidrule(lr){6-7}
& coef. & \multicolumn{1}{c}{s.e.}
& coef. & \multicolumn{1}{c}{s.e.}
& coef. & \multicolumn{1}{c}{s.e.}    \\
\midrule
 Prices         &    $-1.750$ &   (0.019)    &    $-6.519$  &   (0.209)    &  $-12.001$  & (0.777)\\
 Size           &    0.037 &    (0.001)   &    0.018 &   (0.001)    &  $-0.060$  & (0.013) \\
 Light          &    0.259  &   (0.010)  &    0.413 &   (0.014)    &  $-0.270$  & (0.144) \\
 Plain   &    0.508 &   (0.007)   &    0.423  &   (0.009)   &  0.439 & (0.012) \\
 log(\#Flavors)   &    1.127  &   (0.004)  &    1.106 &   (0.005)    &  1.135    & (0.007) \\
 Income $\times$ price &      &       &        &      &  4.333   & (0.378)\\
 Income $\times$ light &     &        &        &      &  0.215  & (0.069)\\
Age $\times$ light    &      &       &      &        & $-0.565$  & (0.113)  \\
 Age $\times$ size     &    &         &   &           & $-0.067$& (0.008)  \\
\midrule 
 Own price elasticity-mean       & \multicolumn{2}{c}{-1.32}  & \multicolumn{2}{c}{-4.917} & \multicolumn{2}{c}{-6.306} \\
 Own price elasticity-median     & \multicolumn{2}{c}{-1.177} & \multicolumn{2}{c}{-4.384} & \multicolumn{2}{c}{-6.187} \\
 Diversion outside option-mean   &  \multicolumn{2}{c}{0.72}  &  \multicolumn{2}{c}{0.72}  &  \multicolumn{2}{c}{0.39}  \\
 Diversion outside option-median &  \multicolumn{2}{c}{0.71}  &  \multicolumn{2}{c}{0.71}  &  \multicolumn{2}{c}{0.38}  \\
\bottomrule
\end{widetable}
\label{Tab:demand}
\end{table}
 \begin{tablenotes}
 \item[] \footnotesize{In the table, we report demand estimates for a logit model of demand obtained from OLS estimation in column 1 and 2SLS  estimation in column 2. Column 3 corresponds to the full BLP model. All specifications have fixed effects for quarter, store and brand and are estimated with 205,123 observations.} 
\end{tablenotes}

%\begin{table}[!h]\footnotesize
%    \centering\caption{Markups Summary Stat}
%    \input{MarkupDescTable}
%\end{table}

%\begin{figure}[!h]
%    \centering\caption{Markups Distribution}
%    \subfloat[IV1]{\includegraphics[scale=0.5]{MarkupFig1.png}}
%    \subfloat[Mixed 2]{\includegraphics[scale=0.5]{MarkupFig2.png}}
    
%    \label{fig:my_label}
%\end{figure}
