# Supplementary material for: Testing Firm Conduct
Source: arXiv:2301.06720 source file (2024-01-17)
Supplement: Supplementary file 16 [file pyRV.tex]

\begin{figure}[H]
    \centering
    \caption{Code for Demand Estimation and Testing}
    \hspace{-2.5cm}\begin{subfigure}[b]{0.5\textwidth}
          \caption*{\hspace{-1.5cm}Panel A. Demand Estimation Code}
         \includegraphics[scale=0.3, trim={.1cm 0 0 0}, clip]{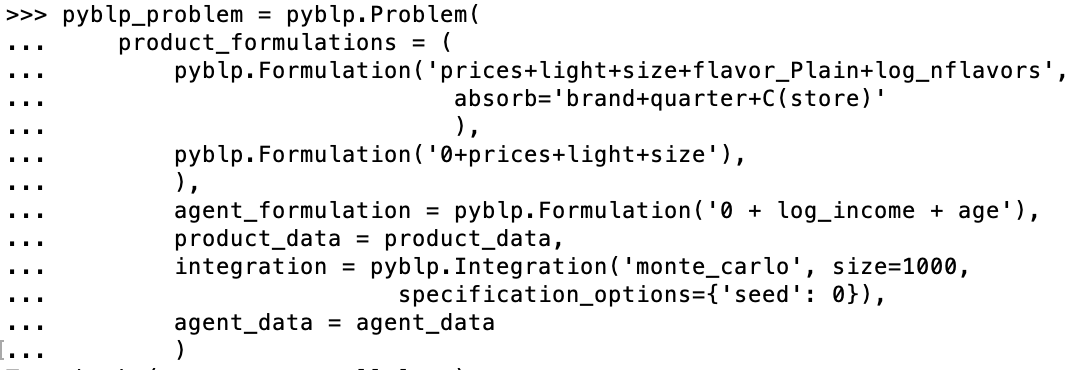}\\
\includegraphics[scale=0.3, trim={.1cm 0 0 0}, clip]{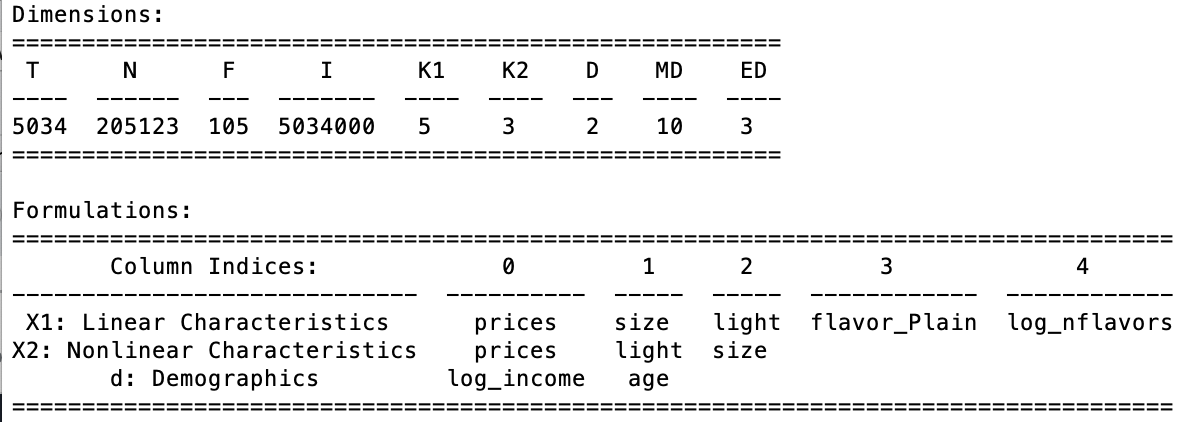}\\
\vspace{1.75cm}
     \end{subfigure}
     \hspace{-1cm}\begin{subfigure}[b]{0.4\textwidth}
        
         \caption*{\hspace{1.5cm}Panel B. Testing Code}
         \includegraphics[scale=0.3]{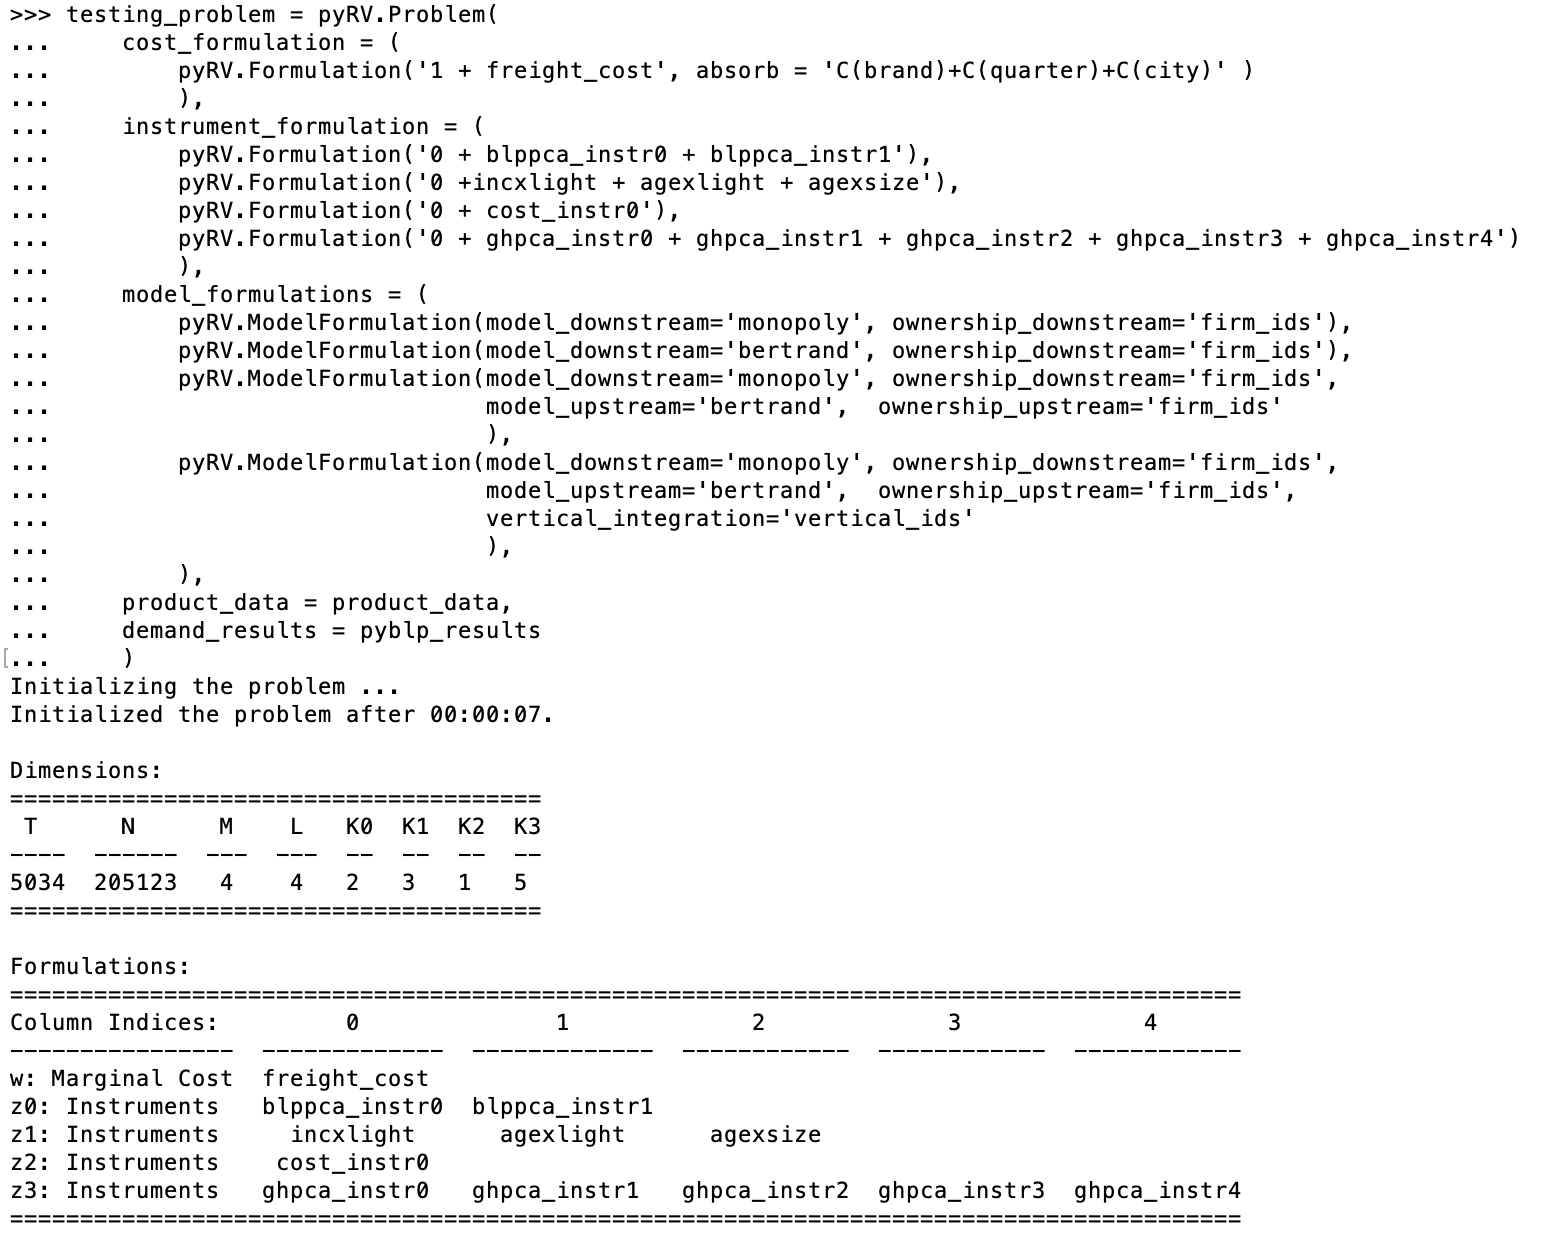}
     \end{subfigure}
    
\subcaption*{Panel A and B respectively report the definition of the demand estimation problem in \texttt{PyBLP} and the testing problem in \texttt{pyRV}. }
\end{figure}
