# Supplementary material for: Testing Firm Conduct
Source: arXiv:2301.06720 source file (2024-01-17)
Supplement: Supplementary file 17 [file OtherAppendixMaterial.tex]

\pagebreak
