# Supplementary material for: Testing Firm Conduct
Source: arXiv:2301.06720 source file (2024-01-17)
Supplement: Supplementary file 28 [file Appendix_StockYogo.tex]

In this appendix we construct the critical values in Table \ref{tab:Tab_StockYogo} for a practical test of degeneracy. To do so, we first  derive asymptotic distributions for the RV test statistic when instrumenst are weak for testing under the assumption of homoskedasticity.\footnote{Similarly to extensions in the weak-IV literature (Montiel-Olea and Pflueger (2013), Lee et al. (2020)), this procedure can be extended to settings with heteroskedasticity. We leave this for future work.} Then, similarly to Stock and Yogo (2005), we use simulations based on the asymptotic distribution to construct critical values for the F statistics of two ad-hoc first stage regressions. Based on these F statistics, we propose a diagnostic that targets worst case rejection probabilities for the RV statistic at or below the nominal size. 


\subsection{Preliminaries}
We start by recapping our setup of weak instruments for testing. Recall our model:
\begin{align*}
    p = \Delta_0 + \omega_0,
\end{align*}
and for model $m$ we define a modified first stage regression:
\begin{align*}
    \Delta_0 - \Delta_m = z(\Gamma^*_0 - \Gamma_m) + e_m.
\end{align*}
Then, we adopt a weak instrument asymptotics similar to \cite{ss97}: $(\hat\Gamma^{*}_0-\hat\Gamma_m) = \frac{q_m}{\sqrt{n}} + o_p(n^{-1/2})$ for a finite vector $q_m$. This is a special case of weak instruments for testing as defined in Proposition \ref{prop:degen}. Under this weak instruments for testing asymptotics, we have:
\begin{align}
\frac{z'\omega_0}{\sqrt{n}} &\rightarrow_d \xi_{\omega_0}\\
\frac{z'e_m}{\sqrt{n}} &\rightarrow_d \xi_{e_m}\\ 
%\frac{z'p}{\sqrt{n}}&=\frac{z'\Delta_0^* +z'e_0^* + z'\omega_0 }{\sqrt{n}}\\ &\rightarrow_d A_{zz}'c^*_0 + \xi_{e^*_0} + \xi_{\omega_0}\\
\frac{z'(\Delta_0 - \Delta_m)}{\sqrt{n}} &\rightarrow_d A_{zz}q_m + \xi_{e_m}\\
\frac{z'(p-\Delta_m)}{\sqrt{n}} &\rightarrow_d A_{zz}q_m + \xi_{e_m}+ \xi_{\omega_0}\\
\hat A_{zz}^{-1/2}\frac{z'(p-\Delta_m)}{\sqrt{n}} &\rightarrow_d A_{zz}^{1/2} q_m + A_{zz}^{-1/2}\bigg(\xi_{e_m}+ \xi_{\omega_0}\bigg)\\
&= D_m
%\Delta'z(z'z)^{-1}z'\Delta &\rightarrow_d ((A_{zz} C + \xi_e)' A^{-1}_{zz}(A_{zz} C + \xi_e))\\
%\hat\theta_{2SLS} &\rightarrow_d ((A_{zz} C + \xi_e)' A^{-1}_{zz}(A_{zz} C + \xi_e))^{-1}((A_{zz} C + \xi_e)' A^{-1}_{zz}(A_{zz} c^*_0 + \xi_{e^*_0}))\\
%&\qquad + ((A_{zz} C + \xi_e)' A^{-1}_{zz}(A_{zz} C + \xi_e))^{-1}((A_{zz} C + \xi_e)' A^{-1}_{zz}\xi_{\omega_0})
\end{align}
where, if we denote $\xi = (\xi_{\omega_0},\xi_{e_1},\xi_{e_2})$ and $u = (\omega_0, e_1, e_2)$ then $vec(\xi) \sim N(0,E[u_i u_i' \otimes z_i z_i'])$. We also define $$E[u_iu_i'] = \begin{bmatrix} \sigma^2_{\omega_0} & 
\sigma_{\omega_0e_1} &
\sigma_{\omega_0e_2} \\  
\sigma_{\omega_0e_1} &  
\sigma^2_{e_1} &
\sigma_{e_1e_2}\\
\sigma_{\omega_0e_2} & 
\sigma_{e_1e_2} &
\sigma^2_{e_2}
\end{bmatrix}.
$$

Thus, letting $D = (D_1,D_2)'$, the joint distribution of $D$ is given as $D \sim N( D_0 , V)$
where $D_0 = (A_{zz}^{1/2} q_1,A_{zz}^{1/2} q_2)'$ and $$V = \begin{bmatrix}
\sigma^2_{\omega_0} + \sigma^2_{e_1} + 2 \sigma_{\omega_0 e_1} &\sigma^2_{\omega_0} + \sigma_{\omega_0 e_1}+ \sigma_{\omega_0 e_2} + \sigma_{e_1 e_2} \\
\sigma^2_{\omega_0} + \sigma_{\omega_0 e_1}+ \sigma_{\omega_0 e_2} + \sigma_{e_1 e_2} & \sigma^2_{\omega_0} + \sigma^2_{e_2} + 2 \sigma_{\omega_0 e_2}
\end{bmatrix}\otimes I_{d_z}$$.
\subsection{Asymptotic Distribution of the Test Statistic under Weak Instruments for Testing}
With the preliminaries defined, we now use them to derive the distribution of the RV test statistic under a weak instruments for testing asymptotic.  We first consider the numerator of $T^{RV}$.  First note the following:
\begin{align*}
   Q_1 - Q_2 
&= (g_1-g_2)'W(g_1+g_2)\\
&= \frac{1}{n}\bigg((p-\Delta_1)-(p-\Delta_2)\bigg)'z(z'z)^{-1}z'\bigg(p - \Delta_1 +(p-\Delta_2)\bigg)\\
&= \bigg(\frac{(p-\Delta_1)'z}{n}\hat A_{zz}^{-1/2}-\frac{(p-\Delta_2)'z}{n}\hat A_{zz}^{-1/2}\bigg)\bigg( \hat A_{zz}^{-1/2}\frac{z'(p - \Delta_1)}{n} + \hat A_{zz}^{-1/2}\frac{z'(p-\Delta_2)}{n}\bigg)
\end{align*}

so that:
\begin{align*}
     n(Q_1 - Q_2) & = \bigg(\frac{(p-\Delta_1)'z}{\sqrt{n}}\hat A_{zz}^{-1/2}-\frac{(p-\Delta_2)'z}{\sqrt{n}}\hat A_{zz}^{-1/2}\bigg)\bigg( \hat A_{zz}^{-1/2}\frac{z'(p - \Delta_1)}{\sqrt{n}} + \hat A_{zz}^{-1/2}\frac{z'(p-\Delta_2)}{\sqrt{n}}\bigg)\\ &\rightarrow_d  (D_1-D_2)'(D_1+D_2)
     %\bigg( A_{zz}c_2 + \xi_{e_2}- A_{zz}c_1 - \xi_{e_1}\bigg)'A_{zz}^{-1}\bigg(2A_{zz}c^*_0 + 2\xi_{e^*_0} + 2\xi_{\omega_0} - A_{zz}c_1 - \xi_{e_1}- A_{zz}c_2 - \xi_{e_2}\bigg)\\
     %&= \bigg( A_{zz}^{1/2}c_2 + A_{zz}^{-1/2}\xi_{e_2}- A_{zz}^{1/2}c_1 - A_{zz}^{-1/2}\xi_{e_1}\bigg)'\\
     %&\qquad \times \bigg(2A_{zz}^{1/2}c^*_0 + 2A_{zz}^{-1/2}\xi_{e^*_0} + 2A_{zz}^{-1/2}\xi_{\omega_0} - A_{zz}^{1/2}c_1 - A_{zz}^{-1/2}\xi_{e_1}- A_{zz}^{1/2}c_2 - A_{zz}^{-1/2}\xi_{e_2}\bigg)\\
     %&= \bigg( \iota_1 - \iota_2 + A_{zz}^{-1/2}\xi_{e_2} -A_{zz}^{-1/2}\xi_{e^*_0} - A_{zz}^{-1/2}\xi_{e_1}+A_{zz}^{-1/2}\xi_{e^*_0}
     %+A_{zz}^{-1/2}\xi_{\omega_0}-A_{zz}^{-1/2}\xi_{\omega_0}\bigg)'\\
     %&\qquad \times \bigg(\iota_1 + \iota_2 + 2A_{zz}^{-1/2}\xi_{e^*_0} + 2A_{zz}^{-1/2}\xi_{\omega_0} - A_{zz}^{-1/2}\xi_{e_1} - A_{zz}^{-1/2}\xi_{e_2}\bigg)\\
\end{align*}



Now we consider the denominator of the test statistic.  In particular, we define an estimator of the asymptotic variance, denoted $\hat \sigma^2_{RV}$, as:\footnote{See \cite{hp11} for the exact asymptotic variance of the RV test statistic without weak instruments.} 
\begin{align}
    \hat\sigma_{RV}^2 
&= 4g_1'\hat A_{zz}^{-1}\Sigma_1 \hat A_{zz}^{-1}g_1 +4g_2'\hat A_{zz}^{-1}\Sigma_2 \hat A_{zz}^{-1} g_2 - 8g_1'\hat A_{zz}^{-1}\Sigma_{1,2} \hat A_{zz}^{-1} g_2.
\end{align}
where
\begin{align}
&\Sigma_m = \frac{1}{n}\sum_{i=1}^n \bigg( z_i\hat \omega_{mi} \bigg) \bigg(z_i \hat\omega_{mi} \bigg)'\label{eq:Sigma_m}\\
%
&\Sigma_{1,2} = \frac{1}{n}\sum_{i=1}^n \bigg( z_i \hat \omega_{1i} \bigg) \bigg( z_i \hat \omega_{2i} \bigg) '
\end{align}

We first examine the convergence of $g_1$ and $g_2$:
\begin{align*}
    \sqrt{n} g_m &= \hat A_{zz}^{1/2} \hat A_{zz}^{-1/2}\frac{z'\Delta^*_0-z'\Delta_m + z'\omega_0}{\sqrt{n}}\\
    &\rightarrow_d A_{zz}^{1/2} \bigg(A_{zz}^{1/2}c^*_0 + A_{zz}^{-1/2}\xi_{e^*_0} + A_{zz}^{-1/2}\xi_{\omega_0} - A_{zz}^{1/2}c_m - A_{zz}^{-1/2}\xi_{e_m}\bigg)\\
        &= A_{zz}^{1/2} D_m
\end{align*}

Now, we examine the convergence of $\Sigma_m$.  In doing so, it is convenient to define $u_{mi} = \omega_{0i}+e_{mi}$:
\begin{align}
       \Sigma_m &= \frac{1}{n}\sum_{i=1}^n ( z_i \hat \omega_m) ( z_i \hat \omega_m)'\\
       %&=\frac{1}{n}\sum_{i=1}^n \bigg( z_i( p_i-\Delta_{mi}) \bigg) \bigg( z_i( p_i-\Delta_{mi}) \bigg)'\\
       &=\frac{1}{n}\sum_{i=1}^n \bigg( z_i( \Delta^*_{0i}+\omega_{0i}-\Delta_{mi}) \bigg) \bigg( z_i(\Delta^*_{0i}+\omega_{0i}-\Delta_{mi}) \bigg)'\\
       &=\frac{1}{n}\sum_{i=1}^n \bigg(  z_iz_{i}'\frac{q_m}{\sqrt{n}}+z_i(e_{mi}+\omega_{0i}) \bigg) \bigg( z_iz_{i}'\frac{q_m}{\sqrt{n}}+z_i(e_{mi}+\omega_{0i}) \bigg)'\\
     %&=\frac{1}{n}\sum_{i=1}^n \bigg(  z_iz_{i}'\frac{q_m}{\sqrt{n}}+z_iu_{mi} \bigg) \bigg( z_iz_{i}'\frac{q_m}{\sqrt{n}}+z_iu_{mi} \bigg)'\\
       &=\frac{1}{n}\sum_{i=1}^n  z_iz_{i}'\frac{q_m}{\sqrt{n}}\frac{q_m'}{\sqrt{n}}z_iz_{i}'+ \frac{1}{n}\sum_{i=1}^n  z_iz_{i}'\frac{q_m}{\sqrt{n}}'u_{mi}z_i'
 +\frac{1}{n}\sum_{i=1}^n z_iu_{mi}'\frac{q_m'}{\sqrt{n}}z_iz_{i}' +\frac{1}{n}\sum_{i=1}^n z_iu_{mi}'u_{mi} z_i'\\
 &\rightarrow_p (\sigma^2_{\omega_0} + \sigma^2_{e_m}  +2\sigma_{\omega_0e_m}) A_{zz}
\end{align}
By similar steps,  $\Sigma_{12}\rightarrow_p (\sigma^2_{\omega_0} + \sigma_{\omega_0e_1} +\sigma_{\omega_0e_2} + \sigma_{e_1e_2}) A_{zz}$.

Thus, the denominator of the RV test converges in distribution as follows:
\begin{align*}
    \hat\sigma^2&=4g_1'\hat A_{zz}^{-1}\Sigma_1 \hat A_{zz}^{-1}g_1 +4g_2'\hat A_{zz}^{-1}\Sigma_2 \hat A_{zz}^{-1} g_2 - 8g_1'\hat A_{zz}^{-1}\Sigma_{1,2} \hat A_{zz}^{-1} g_2\\
    &\rightarrow_d %4\sigma^2_{u_1}D_1'A_{zz}^{1/2} A_{zz}^{-1}A_{zz}A_{zz}^{-1}A_{zz}^{1/2} D_1 + 4\sigma^2_{u_2}D_2'A_{zz}^{1/2} A_{zz}^{-1}A_{zz}A_{zz}^{-1}A_{zz}^{1/2} D_2 - 8\sigma^2_{u_{12}}D_1'A_{zz}^{1/2} A_{zz}^{-1}A_{zz}A_{zz}^{-1}A_{zz}^{1/2} D_2\\
    4\sigma^2_{u_1}D_1'D_1 + 4\sigma^2_{u_2}D_2'D_2 - 8\sigma^2_{u_{12}}D_1'D_2\\
    &= 4 \bigg(D'\begin{bmatrix}I_{d_z} & 0 \\0 &-I_{d_z} \end{bmatrix}V\begin{bmatrix}I_{d_z} &0 \\0 &-I_{d_z} \end{bmatrix}D\bigg)
\end{align*}



Using the convergence results for the numerator and denominator, we can thus construct an asymptotic distribution for the test statistic $T^{RV}$. 
\begin{align}
    T^{RV} &\rightarrow_d\frac{D_1'D_1 - D_2'D_2}{2\sqrt{D'\begin{bmatrix}I_{d_z} & 0 \\0 &-I_{d_z} \end{bmatrix}V\begin{bmatrix}I_{d_z} &0 \\0 &-I_{d_z} \end{bmatrix}D}}
\end{align}

It is useful to consider an equivalent representation of the asymptotic distribution of $T^{RV}$. This representation is based on the rotation proposed in Magnolfi, Soelvsten, and Sullivan (2021). Consider $\pi = (\pi_1,\pi_2)' = (D_1+D_2,D_1-D_2)' = RD$ where $R = \begin{bmatrix} 1 & 1 \\ 1 & -1\end{bmatrix}$.  Thus, the distribution of $\pi$ is given as: $\pi \sim N(R D_0, \Omega)$ where $\Omega = R V R$.  Then we can write $T^{RV}$ as a function of $\pi$.

\begin{align}
    T^{RV} 
  &\rightarrow_d \frac{(D_1+D_2)'(D_1-D_2)}{2\sqrt{D'\begin{bmatrix}I_{d_z} & 0 \\0 &-I_{d_z} \end{bmatrix}V\begin{bmatrix}I_{d_z} &0 \\0 &-I_{d_z} \end{bmatrix}D}} \\ 
      %&= \frac{(D_1'+D_2)'(D_1-D_2)}{2\sqrt{D'\begin{bmatrix}I_{d_z} & I_{d_z}  \\I_{d_z}  &-I_{d_z} \end{bmatrix}\begin{bmatrix}0& I_{d_z}  \\I_{d_z}  &0 \end{bmatrix}\begin{bmatrix}.5I_{dz} &.5I_{dz} \\.5I_{dz} &-.5I_{dz} \end{bmatrix}V\begin{bmatrix}.5I_{dz} &.5I_{dz} \\.5I_{dz} &-.5I_{dz} \end{bmatrix}\begin{bmatrix}0& I_{d_z}  \\I_{d_z}  &0 \end{bmatrix}\begin{bmatrix}I_{d_z} & I_{d_z}  \\I_{d_z}  &-I_{d_z} \end{bmatrix}D}} \\ 
       &= \frac{(D_1+D_2)'(D_1-D_2)}{\sqrt{D'\begin{bmatrix}I_{d_z} & I_{d_z}  \\I_{d_z}  &-I_{d_z} \end{bmatrix}\begin{bmatrix}0& I_{d_z}  \\I_{d_z}  &0 \end{bmatrix}\begin{bmatrix}I_{dz} &I_{dz} \\I_{dz} &-I_{dz} \end{bmatrix}V\begin{bmatrix}I_{dz} &I_{dz} \\I_{dz} &-I_{dz} \end{bmatrix}\begin{bmatrix}0& I_{d_z}  \\I_{d_z}  &0 \end{bmatrix}\begin{bmatrix}I_{d_z} & I_{d_z}  \\I_{d_z}  &-I_{d_z} \end{bmatrix}D}} \\ 
       &= \frac{(D_1+D_2)'(D_1-D_2)}{\sqrt{D'R S_p R V R S_p R D}} \\ 
        &= \frac{\pi_1'\pi_2}{\sqrt{\pi' S_p\Omega S_p \pi}} 
\end{align}
where $S_p = \begin{bmatrix} 0 & I_{d_z} \\ I_{d_z} & 0 \end{bmatrix}$.

It is further useful to standardize $\pi$.  We partition $\Omega$ into four $d_z \times d_z$ block matrices.  Let $\pi^{std} = (\Omega_{11}^{-1/2} \pi_1,\Omega_{22}^{-1/2} \pi_2)\sim N(\pi_0^{std}, \Omega^{std}\otimes I_{d_z} )$, where $\pi^{std}_{01} =  \Omega_{11}^{-1/2} A^{1/2}_{zz} (q_1 + q_2) $ and $\pi^{std}_{02} =  \Omega_{22}^{-1/2} A^{1/2}_{zz} (q_1 - q_2)$ and  $\Omega^{std} = \begin{bmatrix} 1 & \rho \\ \rho & 1 \end{bmatrix}$, and  $\rho$ is the correlation between $\pi_1^{std}$ and $\pi_2^{std}$. Then we can write the asymptotic distribution of the RV test statistic as a function of $\pi^{std}$.

%\begin{align}
%    V^{std} &= \begin{bmatrix}1 & \rho\\ \rho & 1\end{bmatrix}\\
%    &= \begin{bmatrix}V_{11}^{-1/2} & 0 \\ 0 & V_{22}^{-1/2}\end{bmatrix} \begin{bmatrix}V_{11} & V_{12}\\ V_{12} & V_{22}\end{bmatrix} \begin{bmatrix}V_{11}^{-1/2} & 0 \\ 0 & V_{22}^{-1/2}\end{bmatrix}\\
%    &= S_VVS_V
%\end{align}
%so that 
%\begin{align}V &= \begin{bmatrix}V_{11}^{1/2} & 0 \\ 0 & V_{22}^{1/2}\end{bmatrix} \begin{bmatrix} 1& \rho \\ \rho & 1\end{bmatrix} \begin{bmatrix}V_{11}^{1/2} & 0 \\ 0 & V_{22}^{1/2}\end{bmatrix}\\
%&=S_V^{-1} V^{std} S_V^{-1}\end{align}

\begin{align}
     \frac{\pi_1'\pi_2}{\sqrt{\pi' S_p\Omega S_p \pi}} 
    &= \frac{\pi_1'\pi_2}{\sqrt{\pi' S_p\begin{bmatrix}\Omega_{11}^{1/2} I_{dz} & 0 \\ 0 & \Omega_{22}^{1/2} I_{dz}\end{bmatrix}\Omega^{std} \begin{bmatrix}\Omega_{11}^{1/2} I_{dz} & 0 \\ 0 & \Omega_{22}^{1/2} I_{dz}\end{bmatrix}S_p \pi}} \\
    %&= \frac{\pi_1'\pi_2}{\sqrt{\pi' S_p S^{-1}_\Omega\Omega^{std} S^{-1}_\Omega S_p \pi}} \\
    &= \frac{\pi_1'\pi_2}{\sqrt{\begin{bmatrix}\Omega_{11}^{1/2} \pi_2'  &  \Omega_{22}^{1/2} \pi_1'  \end{bmatrix}\Omega^{std} \begin{bmatrix}  \Omega_{11}^{1/2} \pi_2\\ \Omega_{22}^{1/2} \pi_1  \end{bmatrix}}} \\
        &=\frac{\Omega_{11}^{-1/2}\Omega_{22}^{-1/2}}{\Omega_{11}^{-1/2}\Omega_{22}^{-1/2}} \frac{\pi_1'\pi_2}{\sqrt{\begin{bmatrix}\Omega_{11}^{1/2} \pi_2'  &  \Omega_{22}^{1/2} \pi_1'  \end{bmatrix}\Omega^{std} \begin{bmatrix}  \Omega_{11}^{1/2} \pi_2\\ \Omega_{22}^{1/2} \pi_1  \end{bmatrix}}} \\
                %&=\frac{\pi_1^{std}'\pi_2^{std}}{\sqrt{\begin{bmatrix}\Omega_{22}^{-1/2} \pi_2'  &  \Omega_{11}^{-1/2} \pi_1'  \end{bmatrix}\Omega^{std} \begin{bmatrix}  \Omega_{22}^{-1/2} \pi_2\\ \Omega_{11}^{-1/2} \pi_1  \end{bmatrix}}} \\
                &=\frac{\pi_1^{std}'\pi_2^{std}}{\sqrt{\begin{bmatrix}\Omega_{11}^{-1/2} \pi_1 \\\Omega_{22}^{-1/2} \pi_2    \end{bmatrix}'S_p\Omega^{std} S_p\begin{bmatrix}  \Omega_{11}^{-1/2} \pi_1 \\\Omega_{22}^{-1/2} \pi_2 \end{bmatrix}}}\\          %&=\frac{\pi_1^{std}'\pi_2^{std}}{\sqrt{(S_\Omega\pi)'S_p\Omega^{std} S_\Omega\pi}}\\
     &=\frac{\pi_1^{std}'\pi_2^{std}}{\sqrt{\pi^{std}'S_p\Omega^{std} S_p\pi^{std}}}
\end{align}
Finally,
\begin{align}
    T^{RV} \rightarrow_d \frac{\pi_1^{std}'\pi_2^{std}}{\sqrt{\pi^{std}'S_p\Omega^{std} S_p\pi^{std}}}
\end{align}

%$V = \begin{bmatrix}
%\sigma^2_{\omega_0} + \sigma^2_{e_1} + 2 \sigma_{\omega_0 e_1} &\sigma^2_{\omega_0} + \sigma_{\omega_0 e_1}+ \sigma_{\omega_0 e_2} + \sigma_{e_1 e_2} \\
%\sigma^2_{\omega_0} + \sigma_{\omega_0 e_1}+ \sigma_{\omega_0 e_2} + \sigma_{e_1 e_2} & \sigma^2_{\omega_0} + \sigma^2_{e_2} + 2 \sigma_{\omega_0 e_2}
%\end{bmatrix}\otimes I_{d_z}$
%\begin{align}
%    \Omega &= RVR\\
 %   &= R \begin{bmatrix}
%\sigma^2_{\omega_0} + \sigma^2_{e_1} + 2 \sigma_{\omega_0 e_1} &\sigma^2_{\omega_0} + \sigma_{\omega_0 e_1}+ \sigma_{\omega_0 e_2} + \sigma_{e_1 e_2} \\
%\sigma^2_{\omega_0} + \sigma_{\omega_0 e_1}+ \sigma_{\omega_0 e_2} + \sigma_{e_1 e_2} & \sigma^2_{\omega_0} + \sigma^2_{e_2} + 2 \sigma_{\omega_0 e_2}
%\end{bmatrix}\otimes I_{d_z} R\\
%&=  \begin{bmatrix}
%2\sigma^2_{\omega_0} + \sigma^2_{e_1} + 3  \sigma_{\omega_0 e_1} + \sigma_{\omega_0 e_2} + \sigma_{e_1 e_2} &2\sigma^2_{\omega_0} + \sigma^2_{e_2} + \sigma_{\omega_0 e_1}+ 3\sigma_{\omega_0 e_2} + \sigma_{e_1 e_2} \\
%\sigma^2_{e_1}+ \sigma_{\omega_0 e_1}- \sigma_{\omega_0 e_2} - \sigma_{e_1 e_2} & -\sigma^2_{e_2} -  \sigma_{\omega_0 e_2} + \sigma_{\omega_0 e_1} + \sigma_{e_1e_2}
%\end{bmatrix}\otimes I_{d_z}R\\
%&=  \begin{bmatrix}
%4\sigma^2_{\omega_0} + \sigma^2_{e_1} + \sigma^2_{e_2} + 4  \sigma_{\omega_0 e_1} + 4 \sigma_{\omega_0 e_2} + 2\sigma_{e_1 e_2} &\sigma^2_{e_1} - \sigma^2_{e_2} + 2\sigma_{\omega_0 e_1}-2\sigma_{\omega_0 e_2}  \\
%\sigma^2_{e_1} - \sigma^2_{e_2} + 2\sigma_{\omega_0 e_1}-2\sigma_{\omega_0 e_2}& \sigma^2_{e_1} +  \sigma^2_{e_2} - 2 \sigma_{e_1e_2}
%\end{bmatrix}\otimes I_{d_z}
%\end{align}
Notice that the asymptotic distribution of the  RV test statistic depends on three paramaters, $\pi_{01}, \pi_{02}$, and $\rho$. The null space in this parameterization is characterized by either $\pi_1 = 0$ or $\pi_2 = 0$.  In the null space, but far from the origin, instruments are relatively strong and the RV test statistic converges to a standard normal.  However, close to the origin, the RV test suffers from a size distortion due to degeneracy.   

\subsection{Deriving the Critical Values}

Using this asymptotic distribution we find thresholds for concentration parameters according to the procedure in Stock and Yogo (2005), which finds critical values for the first stage F-statistic which ensure that inference is reliable. In particular, we are looking for values of $\pi_0^* = (\pi^*_{01},\pi^*_{02})$ such that:
\begin{align}\label{eq:iota_star}
    \Pr[\mid T^{RV}\mid>1.96 \mid \pi_0 =\pi_0^*] = r,
\end{align}
where $r$ is the minimal rejection probability of the test that we are willing to accept.  Here, we depart from Stock and Yogo (2005).  In their context, weak instruments may cause a Wald test to reject more than the nominal size.  Extensive power simulations suggest that in our setting, weak instruments for testing cause the test to be undersized in part of the null space, and to have virtually no power to detect alternatives near that region.  Hence, we choose in Equation (\ref{eq:iota_star}) to target a minimal rejection probability below the nominal size of the test (ie $r\leq 0.05$).    

For a given choice of $r$, we can find $\pi_0^*$ via numerical inversion of Equation (\ref{eq:iota_star}) which involves simulating the probability using the asymptotic distribution of $T^{RV}$ under weak instruments derived above.  Notice that the vector $\pi_0$ has dimension $2 d_z,$ so that solving equation (\ref{eq:iota_star}) potentially involves a high-dimensional search. However, we find that the concentration parameters that determines instrument strength, given by $\mu_{1} = \pi_{01}'\pi_{01}$ and  $\mu_2 = \pi_{02}'\pi_{02}$ characterizes well the distribution of the test statistic. As $\mu_1$ and $\mu_2$ are scalars, we can then search over a grid of their values.  For each pair $(\mu_1,\mu_2)$ we solve for a vector $\pi_0$ which rationalizes these concentration parameters.

The distribution of the RV statistic also depends on $\rho$.  For each guess of the concentration parameter, we evaluate the probability over a fine grid of $\rho$ from -1 to 1 by steps of 0.05.  To obtain conservative thresholds, we focus on the worst case rejection probability across $\rho$'s. Thus, instead of inverting Equation (\ref{eq:iota_star}), we invert the following:
$$P(\mu^*) = \min_\rho \Pr[\mid T^{RV} > 1.96\mid \mu = \mu^*, \rho] = r$$

  
We further refine our search based on simulation evidence.  In Figure \ref{fig:power_SY} we plot the contour sets of worst case rejection probabilities in the space of $(\mu_1, \mu_2)$ obtained from 100,000 simulations.  For illustrative purposes, we do so in the case of one instrument.  Simulations with more than one instrument are qualitatively similar.     

 \begin{figure}[ht]
     \centering
      \caption{Selecting Concentration Parameters}
     \includegraphics[scale = 0.75]{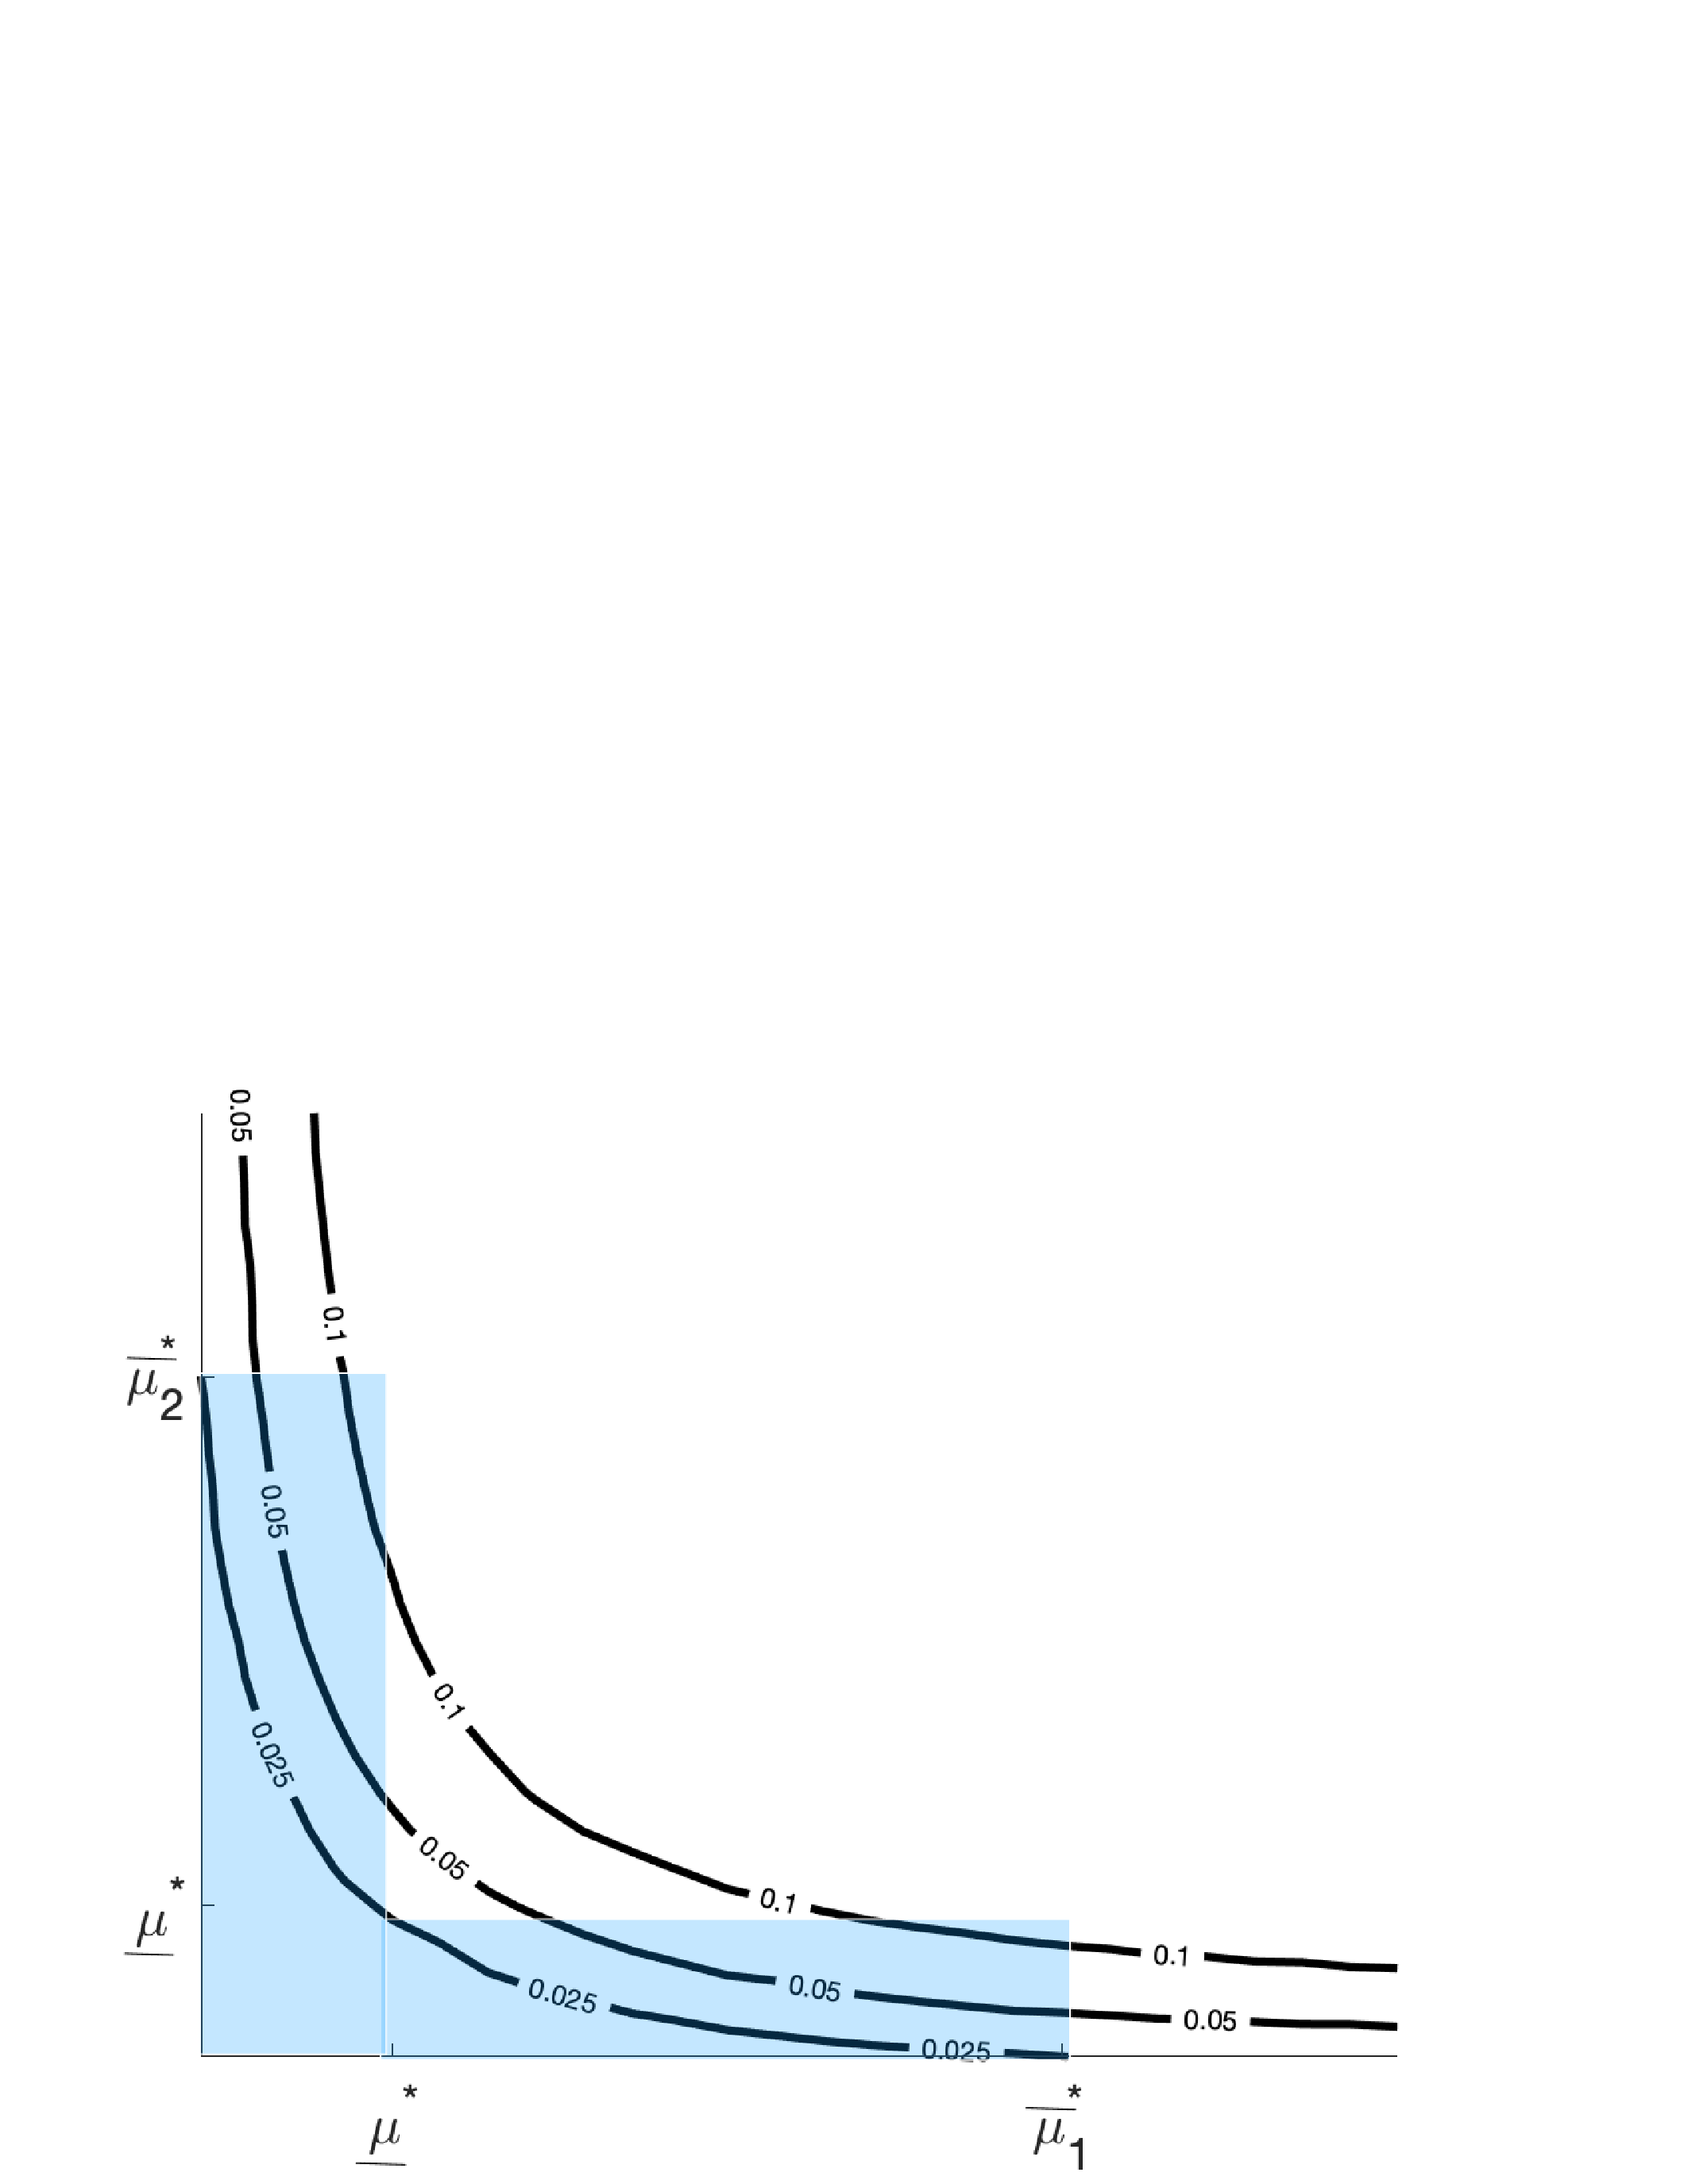}
    \label{fig:power_SY}
    \caption*{\footnotesize{This figure illustrates in the space of concentration parameters $\mu_1$ and $\mu_2$ our criterion for choosing threshold values $\mu^*$.  The black curves are contour sets of worst case rejection probabilities for the RV test.  The shaded L-shaped region indicates our conservative characterization of the region of degeneracy for a minimal size of 0.025.}}
\end{figure}

As shown in the figure, degeneracy manifests itself in two ways: (i) the test is undersized in the part of the null space (represented by the $x-$ and $y-$ axis) close to the origin and (ii) the test has very low power for alternatives close to the origin.  While it is possible to exactly characterize the region below any contour, we choose to approximate that region with a simple L-shaped area.  Specifically, the area is characterized by the threshold values $\overline{\mu}^*_1$ and $\overline{\mu}^*_2$ where the contour corresponding to rejection probability $r$ intersects the $x-$ and $y-$ axis respectively as well as the threshold value $\underline{\mu}^*$ where the 45-degree line intersects the contour.  This simple characterization will result in a test of weak instruments for testing which is easy to implement as will be seen below.  We further simplify the definition of the L-shaped region by considering $\overline{\mu}^* = \max\{\overline{\mu}^*_1,\overline{\mu}^*_2\}.$ While this makes our region more conservative, we find across simulations that the values of $\overline{\mu}^*_1$ and $\overline{\mu}^*_2$ are nearly identical.  Formally then, the approximate region of degeneracy is defined as: \begin{align}\label{eq:degen_region}
R = \bigg\{(\mu_1,\mu_2)\, \bigg\vert\, \min\{\mu_1,\mu_2\} \leq \underline{\mu}^* \text{ AND } \max\{\mu_1,\mu_2\} \leq \overline{\mu}^*   \bigg\} 
\end{align}


$R$ is characterized by two values $\underline{\mu}^*$ and $\overline{\mu}^*$.  We solve for $\underline{\mu}^*$ by searching along the 45-degree line in steps of 0.1, starting at the origin.  We denote $\underline{\mu}^*$ as the lowest value of $\mu$ for which the estimate of $P(\mu)$ obtained from 100,000 simulations equals $r$ .  Similarly, we search along the $x-$ and $y-$ axis in steps of 1, obtaining $\overline{\mu}^*_1$ and $\overline{\mu}^*_2$. We set $\overline{\mu}^* = \max\{\overline{\mu}^*_1,\overline{\mu}^*_2\}$.    

While we cannot estimate $\mu$ in the data, it is possible to test the hypothesis that $\mu$ is on the boundary of $R$ using F-statistics.  Specifically, we can compute F-statistics for two regressions (i) $2p-\Delta_1-\Delta_2$  on instruments and (ii) $\Delta_1-\Delta_2$ on instruments as follows, letting the residuals from these regressions be $\hat\zeta_1$ and $\hat\zeta_2$ respectively. 
\begin{align*}
    F_1 &= \frac{((z'z)^{-1}z'(2\Delta_0+2\omega_0-\Delta_1-\Delta_2))'z'z((z'z)^{-1}z'(z(2\Delta_0+2\omega_0-\Delta_1-\Delta_2))}{d_z\hat\sigma^2_{\zeta_1}},\\
&=    \frac{((z'z)^{-1}z'(z\frac{q_1+q_2}{\sqrt{n}}+\zeta_1))'z'z((z'z)^{-1}z'(z\frac{q_1+q_2}{\sqrt{n}}+\zeta_1))}{d_z\hat\sigma^2_{\zeta_1}},\\
&= \frac{ ( \hat A_{zz}^{1/2}(q_1+q_2)\hat A_{zz}^{-1/2}\frac{z'\zeta_1}{\sqrt{n}})'( \hat A_{zz}^{1/2}(q_1+q_2)+\hat A_{zz}^{-1/2}\frac{z'\zeta_1}{\sqrt{n}})}{d_z\hat\sigma^2_{\zeta_1}},\\
&= \frac{( \hat A_{zz}^{1/2}(q_1+q_2)+\hat A_{zz}^{-1/2}\frac{z'\zeta_1}{\sqrt{n}})'}{\sqrt{d_z}\hat\sigma_{\zeta_1}}\frac{( \hat A_{zz}^{1/2}(q_1+q_2)+\hat A_{zz}^{-1/2}\frac{z'\zeta_1}{\sqrt{n}})}{\sqrt{d_z}\hat\sigma_{\zeta_1}},\\
 d_z F_1&\rightarrow_d \chi^2_{d_z}(\pi_{01}'\pi_{01})
\end{align*}
where $\zeta_1=2\omega_0 + e_1 + e_2$ and $\sigma^2_{\zeta_1} = 4\sigma^2_{\omega_0} + \sigma^2_{e_1} + \sigma^2_{e_2} + 4\sigma_{\omega_0 e_1} + 4\sigma_{\omega_0 e_2} + 2\sigma_{e_1 e_2}=\Omega_{11}$.

Also, 
\begin{align*}
    F_2 &= \frac{(\hat\Gamma_1-\hat\Gamma_2)'z'z(\hat\Gamma_1-\hat\Gamma_2)}{d_z\hat\sigma^2_{\zeta_2}},\\
&=    \frac{((z'z)^{-1}z'(\Delta_1-\Delta_2))'z'z((z'z)^{-1}z'(z(\Delta_1-\Delta_2))}{d_z\hat\sigma^2_{\zeta_2}},\\
&=    \frac{((z'z)^{-1}z'(z\frac{q_1-q_2}{\sqrt{n}}+\zeta_2))'z'z((z'z)^{-1}z'(z\frac{q_1-q_2}{\sqrt{n}}+\zeta_2))}{d_z\hat\sigma^2_{\zeta_2}},\\
&= \frac{ ( \hat A_{zz}^{1/2}(q_1-q_2)+\hat A_{zz}^{-1/2}\frac{z'\zeta_2}{\sqrt{n}})'( \hat A_{zz}^{1/2}(q_1-q_2)+\hat A_{zz}^{-1/2}\frac{z'\zeta_2}{\sqrt{n}})}{d_z\hat\sigma^2_{\zeta_2}},\\
&= \frac{( \hat A_{zz}^{1/2}(q_1-q_2)+\hat A_{zz}^{-1/2}\frac{z'\zeta_2}{\sqrt{n}})'}{\sqrt{d_z}\hat\sigma_{\zeta_2}}\frac{( \hat A_{zz}^{1/2}(q_1-q_2)+\hat A_{zz}^{-1/2}\frac{z'\zeta_2}{\sqrt{n}})}{\sqrt{d_z}\hat\sigma_{\zeta_2}},\\
 d_z F_2&\rightarrow_d \chi^2_{d_z}(\pi_{02}'\pi_{02})
\end{align*}

 We can find two critical values $\underline{cv}$ and $\overline{cv}$ corresponding to tests of the null that  $\mu_i = \underline{\mu}^*$ and $\mu_i = \overline{\mu}^*$ that have nominal size 0.05.
 As the distribution of $F_1$ and $F_2$ are identical up to the non-centrality, we write generically:
\begin{align*}
\Pr[F_i \geq \underline{cv} \mid \mu_i = \underline{\mu}^*]&=    \Pr[d_z F \geq d_z \underline{cv} \mid \mu = \underline{\mu}^*]\\ 
    &\rightarrow_p \Pr[\chi_{d_z}^2(\underline{\mu}^*) \geq d_z \underline{cv} ]\\
    &=1-G\bigg( d_z \underline{cv},\underline{\mu}^*\bigg)\\
    &= 0.05
\end{align*}
where $G$ is the cdf of a non-central $\chi_{d_z}^2$ distribution. So, we can invert to get the critical value as:
$$\underline{cv} = \frac{1}{d_z}G^{-1}(0.95,\underline{\mu}^*).$$
Notice that $\overline{cv}$ can be obtained in an analogous way.  

We then construct a rejection region that mimics the shape of the region of degeneracy $R$.  Specifically, we reject weak instruments for testing if either of the two conditions are satisfied: (i) $\min\{F_1,F_2\} > \underline{cv}$ or (ii) $\max\{F_1,F_2\} > \overline{cv}$.  We argue that, when $\mu$ is on the boundary of $R$, this procedure rejects in favor of the one-sided alternative that $\mu \not\in R$ with probability = 0.05.  Specifically, assuming that $\mu$ lies on the boundary of $R$, there are four cases that can obtain: (i) $\mu_1 = \overline{\mu}^*$ and $\mu_2 < \underline{\mu}^*$, (ii)  $\mu_1 = \underline{\mu}^*$ and $\mu_2 < \overline{\mu}^*$, (iii)  $\mu_1 < \overline{\mu}^*$ and $\mu_2 = \underline{\mu}^*$, and (iv) $\mu_1 < \underline{\mu}^*$ and $\mu_2 = \overline{\mu}^*$.  In each of these cases, only one condition is binding.  Hence, asymptotically, rejection occurs in case (i) when $F_1 > \overline{cv}$, in case (ii) when $F_1>\underline{cv}$, in case (iii) when $F_2 > \underline{cv}$, in case (iv) when $F_2>\overline{cv}$. In each of these cases, asymptotically our test has the desired size.  As the values of $\mu^*$ and therefore the critical values depend on $r$ and $d_z$, we report in Table \ref{tab:Tab_StockYogo} critical values for $r = 0.01$, 0.025, and 0.05, and for $dz \in [1,29]$.  Simulations show that this procedure is conservative, but valid. 
