# Supplementary material for: Testing Firm Conduct
Source: arXiv:2301.06720 source file (2024-01-17)
Supplement: Supplementary file 29 [file Appendix_StockYogo_Size.tex]

In this appendix we construct the critical values in Table \ref{tab:Tab_StockYogo} for a practical test of degeneracy. To do so, we first  derive asymptotic distributions for the RV test statistic when instrumenst are weak for testing under the assumption of homoskedasticity.\footnote{Similarly to extensions in the weak-IV literature (Montiel-Olea and Pflueger (2013), Lee et al. (2020)), this procedure can be extended to settings with heteroskedasticity. We leave this for future work.} Then, similarly to Stock and Yogo (2005), we use simulations based on the asymptotic distribution to construct critical values for the F statistics of two ad-hoc first stage regressions. Based on these F statistics, we propose a diagnostic that targets worst case size distortions for the RV statistic above the nominal size. 


\subsection{Preliminaries}
We start by recapping our setup of weak instruments for testing. Recall our model:
\begin{align*}
    p = \Delta_0 + \omega_0,
\end{align*}
and for model $m$ we define a modified first stage regression:
\begin{align*}
    \Delta_0 - \Delta_m = z(\Gamma^*_0 - \Gamma_m) + e_m.
\end{align*}
Then, we adopt a weak instrument asymptotics similar to \cite{ss97}: $(\hat\Gamma^{*}_0-\hat\Gamma_m) = \frac{q_m}{\sqrt{n}} + o_p(n^{-1/2})$ for a finite vector $q_m$. This is a special case of weak instruments for testing as defined in Proposition \ref{prop:degen}. Under this weak instruments for testing asymptotics, we have:
\begin{align}
\frac{z'\omega_0}{\sqrt{n}} &\rightarrow_d \xi_{\omega_0}\\
\frac{z'e_m}{\sqrt{n}} &\rightarrow_d \xi_{e_m}\\ 
%\frac{z'p}{\sqrt{n}}&=\frac{z'\Delta_0^* +z'e_0^* + z'\omega_0 }{\sqrt{n}}\\ &\rightarrow_d A_{zz}'c^*_0 + \xi_{e^*_0} + \xi_{\omega_0}\\
\frac{z'(\Delta_0 - \Delta_m)}{\sqrt{n}} &\rightarrow_d A_{zz}q_m + \xi_{e_m}\\
\frac{z'(p-\Delta_m)}{\sqrt{n}} &\rightarrow_d A_{zz}q_m + \xi_{e_m}+ \xi_{\omega_0}\\
\hat A_{zz}^{-1/2}\frac{z'(p-\Delta_m)}{\sqrt{n}} &\rightarrow_d A_{zz}^{1/2} q_m + A_{zz}^{-1/2}\bigg(\xi_{e_m}+ \xi_{\omega_0}\bigg)\\
&= D_m
%\Delta'z(z'z)^{-1}z'\Delta &\rightarrow_d ((A_{zz} C + \xi_e)' A^{-1}_{zz}(A_{zz} C + \xi_e))\\
%\hat\theta_{2SLS} &\rightarrow_d ((A_{zz} C + \xi_e)' A^{-1}_{zz}(A_{zz} C + \xi_e))^{-1}((A_{zz} C + \xi_e)' A^{-1}_{zz}(A_{zz} c^*_0 + \xi_{e^*_0}))\\
%&\qquad + ((A_{zz} C + \xi_e)' A^{-1}_{zz}(A_{zz} C + \xi_e))^{-1}((A_{zz} C + \xi_e)' A^{-1}_{zz}\xi_{\omega_0})
\end{align}
where, if we denote $\xi = (\xi_{\omega_0},\xi_{e_1},\xi_{e_2})$ and $u = (\omega_0, e_1, e_2)$ then $vec(\xi) \sim N(0,E[u_i u_i' \otimes z_i z_i'])$. We also define $$E[u_iu_i'] = \begin{bmatrix} \sigma^2_{\omega_0} & 
\sigma_{\omega_0e_1} &
\sigma_{\omega_0e_2} \\  
\sigma_{\omega_0e_1} &  
\sigma^2_{e_1} &
\sigma_{e_1e_2}\\
\sigma_{\omega_0e_2} & 
\sigma_{e_1e_2} &
\sigma^2_{e_2}
\end{bmatrix}.
$$

Thus, letting $D = (D_1,D_2)'$, the joint distribution of $D$ is given as $D \sim N( D_0 , V)$
where $D_0 = (A_{zz}^{1/2} q_1,A_{zz}^{1/2} q_2)'$ and \begin{align*}
  V &= \begin{bmatrix}
\sigma^2_{\omega_0} + \sigma^2_{e_1} + 2 \sigma_{\omega_0 e_1} &\sigma^2_{\omega_0} + \sigma_{\omega_0 e_1}+ \sigma_{\omega_0 e_2} + \sigma_{e_1 e_2} \\
\sigma^2_{\omega_0} + \sigma_{\omega_0 e_1}+ \sigma_{\omega_0 e_2} + \sigma_{e_1 e_2} & \sigma^2_{\omega_0} + \sigma^2_{e_2} + 2 \sigma_{\omega_0 e_2}
\end{bmatrix}\otimes I_{d_z} \\ 
&=
\bigg(\begin{bmatrix}
1 & 1 & 0\\1&0&1
\end{bmatrix}
E[u_iu_i']
\begin{bmatrix}
1 & 1\\
1 & 0\\
0 & 1
\end{bmatrix}\bigg)\otimes I_{d_z}\\
&= (U'E[u_iu_i']U)\otimes I_{d_z}
\end{align*}

\subsection{Asymptotic Distribution of the Test Statistic under Weak Instruments for Testing}
With the preliminaries defined, we now use them to derive the distribution of the RV test statistic under a weak instruments for testing asymptotic.  We first consider the numerator of $T^{RV}$.  First note the following:
\begin{align*}
   Q_1 - Q_2 
&= (g_1-g_2)'W(g_1+g_2)\\
&= \frac{1}{n}\bigg((p-\Delta_1)-(p-\Delta_2)\bigg)'z(z'z)^{-1}z'\bigg(p - \Delta_1 +(p-\Delta_2)\bigg)\\
&= \bigg(\frac{(p-\Delta_1)'z}{n}\hat A_{zz}^{-1/2}-\frac{(p-\Delta_2)'z}{n}\hat A_{zz}^{-1/2}\bigg)\bigg( \hat A_{zz}^{-1/2}\frac{z'(p - \Delta_1)}{n} + \hat A_{zz}^{-1/2}\frac{z'(p-\Delta_2)}{n}\bigg)
\end{align*}

so that:
\begin{align*}
     n(Q_1 - Q_2) & = \bigg(\frac{(p-\Delta_1)'z}{\sqrt{n}}\hat A_{zz}^{-1/2}-\frac{(p-\Delta_2)'z}{\sqrt{n}}\hat A_{zz}^{-1/2}\bigg)\bigg( \hat A_{zz}^{-1/2}\frac{z'(p - \Delta_1)}{\sqrt{n}} + \hat A_{zz}^{-1/2}\frac{z'(p-\Delta_2)}{\sqrt{n}}\bigg)\\ &\rightarrow_d  (D_1-D_2)'(D_1+D_2)
     %\bigg( A_{zz}c_2 + \xi_{e_2}- A_{zz}c_1 - \xi_{e_1}\bigg)'A_{zz}^{-1}\bigg(2A_{zz}c^*_0 + 2\xi_{e^*_0} + 2\xi_{\omega_0} - A_{zz}c_1 - \xi_{e_1}- A_{zz}c_2 - \xi_{e_2}\bigg)\\
     %&= \bigg( A_{zz}^{1/2}c_2 + A_{zz}^{-1/2}\xi_{e_2}- A_{zz}^{1/2}c_1 - A_{zz}^{-1/2}\xi_{e_1}\bigg)'\\
     %&\qquad \times \bigg(2A_{zz}^{1/2}c^*_0 + 2A_{zz}^{-1/2}\xi_{e^*_0} + 2A_{zz}^{-1/2}\xi_{\omega_0} - A_{zz}^{1/2}c_1 - A_{zz}^{-1/2}\xi_{e_1}- A_{zz}^{1/2}c_2 - A_{zz}^{-1/2}\xi_{e_2}\bigg)\\
     %&= \bigg( \iota_1 - \iota_2 + A_{zz}^{-1/2}\xi_{e_2} -A_{zz}^{-1/2}\xi_{e^*_0} - A_{zz}^{-1/2}\xi_{e_1}+A_{zz}^{-1/2}\xi_{e^*_0}
     %+A_{zz}^{-1/2}\xi_{\omega_0}-A_{zz}^{-1/2}\xi_{\omega_0}\bigg)'\\
     %&\qquad \times \bigg(\iota_1 + \iota_2 + 2A_{zz}^{-1/2}\xi_{e^*_0} + 2A_{zz}^{-1/2}\xi_{\omega_0} - A_{zz}^{-1/2}\xi_{e_1} - A_{zz}^{-1/2}\xi_{e_2}\bigg)\\
\end{align*}



Now we consider the denominator of the test statistic.  In particular, we define an estimator of the asymptotic variance, denoted $\hat \sigma^2_{RV}$, as:\footnote{See \cite{hp11} for the exact asymptotic variance of the RV test statistic without weak instruments.} 
\begin{align}
    \hat\sigma_{RV}^2 
&= 4g_1'\hat A_{zz}^{-1}\Sigma_1 \hat A_{zz}^{-1}g_1 +4g_2'\hat A_{zz}^{-1}\Sigma_2 \hat A_{zz}^{-1} g_2 - 8g_1'\hat A_{zz}^{-1}\Sigma_{1,2} \hat A_{zz}^{-1} g_2.
\end{align}
where
\begin{align}
&\Sigma_m = \frac{1}{n}\sum_{i=1}^n \bigg( z_i\hat \omega_{mi} \bigg) \bigg(z_i \hat\omega_{mi} \bigg)'\label{eq:Sigma_m}\\
%
&\Sigma_{1,2} = \frac{1}{n}\sum_{i=1}^n \bigg( z_i \hat \omega_{1i} \bigg) \bigg( z_i \hat \omega_{2i} \bigg) '
\end{align}

We first examine the convergence of $g_1$ and $g_2$:
\begin{align*}
    \sqrt{n} g_m &= \hat A_{zz}^{1/2} \hat A_{zz}^{-1/2}\frac{z'\Delta^*_0-z'\Delta_m + z'\omega_0}{\sqrt{n}}\\
    &\rightarrow_d A_{zz}^{1/2} \bigg(A_{zz}^{1/2}c^*_0 + A_{zz}^{-1/2}\xi_{e^*_0} + A_{zz}^{-1/2}\xi_{\omega_0} - A_{zz}^{1/2}c_m - A_{zz}^{-1/2}\xi_{e_m}\bigg)\\
        &= A_{zz}^{1/2} D_m
\end{align*}

Now, we examine the convergence of $\Sigma_m$.  In doing so, it is convenient to define $u_{mi} = \omega_{0i}+e_{mi}$:
\begin{align}
       \Sigma_m &= \frac{1}{n}\sum_{i=1}^n ( z_i \hat \omega_m) ( z_i \hat \omega_m)'\\
       %&=\frac{1}{n}\sum_{i=1}^n \bigg( z_i( p_i-\Delta_{mi}) \bigg) \bigg( z_i( p_i-\Delta_{mi}) \bigg)'\\
       &=\frac{1}{n}\sum_{i=1}^n \bigg( z_i( \Delta^*_{0i}+\omega_{0i}-\Delta_{mi}) \bigg) \bigg( z_i(\Delta^*_{0i}+\omega_{0i}-\Delta_{mi}) \bigg)'\\
       &=\frac{1}{n}\sum_{i=1}^n \bigg(  z_iz_{i}'\frac{q_m}{\sqrt{n}}+z_i(e_{mi}+\omega_{0i}) \bigg) \bigg( z_iz_{i}'\frac{q_m}{\sqrt{n}}+z_i(e_{mi}+\omega_{0i}) \bigg)'\\
     %&=\frac{1}{n}\sum_{i=1}^n \bigg(  z_iz_{i}'\frac{q_m}{\sqrt{n}}+z_iu_{mi} \bigg) \bigg( z_iz_{i}'\frac{q_m}{\sqrt{n}}+z_iu_{mi} \bigg)'\\
       &=\frac{1}{n}\sum_{i=1}^n  z_iz_{i}'\frac{q_m}{\sqrt{n}}\frac{q_m'}{\sqrt{n}}z_iz_{i}'+ \frac{1}{n}\sum_{i=1}^n  z_iz_{i}'\frac{q_m}{\sqrt{n}}'u_{mi}z_i'
 +\frac{1}{n}\sum_{i=1}^n z_iu_{mi}'\frac{q_m'}{\sqrt{n}}z_iz_{i}' +\frac{1}{n}\sum_{i=1}^n z_iu_{mi}'u_{mi} z_i'\\
 &\rightarrow_p (\sigma^2_{\omega_0} + \sigma^2_{e_m}  +2\sigma_{\omega_0e_m}) A_{zz}
\end{align}
By similar steps,  $\Sigma_{12}\rightarrow_p (\sigma^2_{\omega_0} + \sigma_{\omega_0e_1} +\sigma_{\omega_0e_2} + \sigma_{e_1e_2}) A_{zz}$.

Thus, the denominator of the RV test converges in distribution as follows:
\begin{align*}
    \hat\sigma^2&=4g_1'\hat A_{zz}^{-1}\Sigma_1 \hat A_{zz}^{-1}g_1 +4g_2'\hat A_{zz}^{-1}\Sigma_2 \hat A_{zz}^{-1} g_2 - 8g_1'\hat A_{zz}^{-1}\Sigma_{1,2} \hat A_{zz}^{-1} g_2\\
    &\rightarrow_d %4\sigma^2_{u_1}D_1'A_{zz}^{1/2} A_{zz}^{-1}A_{zz}A_{zz}^{-1}A_{zz}^{1/2} D_1 + 4\sigma^2_{u_2}D_2'A_{zz}^{1/2} A_{zz}^{-1}A_{zz}A_{zz}^{-1}A_{zz}^{1/2} D_2 - 8\sigma^2_{u_{12}}D_1'A_{zz}^{1/2} A_{zz}^{-1}A_{zz}A_{zz}^{-1}A_{zz}^{1/2} D_2\\
    4\sigma^2_{u_1}D_1'D_1 + 4\sigma^2_{u_2}D_2'D_2 - 8\sigma^2_{u_{12}}D_1'D_2\\
    &= 4 \bigg(D'\begin{bmatrix}I_{d_z} & 0 \\0 &-I_{d_z} \end{bmatrix}V\begin{bmatrix}I_{d_z} &0 \\0 &-I_{d_z} \end{bmatrix}D\bigg)
\end{align*}



Using the convergence results for the numerator and denominator, we can thus construct an asymptotic distribution for the test statistic $T^{RV}$. 
\begin{align}
    T^{RV} &\rightarrow_d\frac{D_1'D_1 - D_2'D_2}{2\sqrt{D'\begin{bmatrix}I_{d_z} & 0 \\0 &-I_{d_z} \end{bmatrix}V\begin{bmatrix}I_{d_z} &0 \\0 &-I_{d_z} \end{bmatrix}D}}
\end{align}



It is useful to consider an equivalent representation of the asymptotic distribution of $T^{RV}$. This representation is based on the rotation proposed in Magnolfi, Soelvsten, and Sullivan (2021). Consider $\pi = (\pi_1,\pi_2)' = (D_1+D_2,D_1-D_2)' = RD$ where $R = \begin{bmatrix} I_{d_z} & I_{d_z} \\ I_{d_z} & -I_{d_z}\end{bmatrix}$.  Thus, the distribution of $\pi$ is given as: $\pi \sim N(R D_0, \Omega)$ where $\Omega = R V R$.  Then we can write $T^{RV}$ as a function of $\pi$.

\begin{align}
    T^{RV} 
  &\rightarrow_d \frac{(D_1+D_2)'(D_1-D_2)}{2\sqrt{D'\begin{bmatrix}I_{d_z} & 0 \\0 &-I_{d_z} \end{bmatrix}V\begin{bmatrix}I_{d_z} &0 \\0 &-I_{d_z} \end{bmatrix}D}} \\ 
      %&= \frac{(D_1'+D_2)'(D_1-D_2)}{2\sqrt{D'\begin{bmatrix}I_{d_z} & I_{d_z}  \\I_{d_z}  &-I_{d_z} \end{bmatrix}\begin{bmatrix}0& I_{d_z}  \\I_{d_z}  &0 \end{bmatrix}\begin{bmatrix}.5I_{dz} &.5I_{dz} \\.5I_{dz} &-.5I_{dz} \end{bmatrix}V\begin{bmatrix}.5I_{dz} &.5I_{dz} \\.5I_{dz} &-.5I_{dz} \end{bmatrix}\begin{bmatrix}0& I_{d_z}  \\I_{d_z}  &0 \end{bmatrix}\begin{bmatrix}I_{d_z} & I_{d_z}  \\I_{d_z}  &-I_{d_z} \end{bmatrix}D}} \\ 
       &= \frac{(D_1+D_2)'(D_1-D_2)}{\sqrt{D'\begin{bmatrix}I_{d_z} & I_{d_z}  \\I_{d_z}  &-I_{d_z} \end{bmatrix}\begin{bmatrix}0& I_{d_z}  \\I_{d_z}  &0 \end{bmatrix}\begin{bmatrix}I_{dz} &I_{dz} \\I_{dz} &-I_{dz} \end{bmatrix}V\begin{bmatrix}I_{dz} &I_{dz} \\I_{dz} &-I_{dz} \end{bmatrix}\begin{bmatrix}0& I_{d_z}  \\I_{d_z}  &0 \end{bmatrix}\begin{bmatrix}I_{d_z} & I_{d_z}  \\I_{d_z}  &-I_{d_z} \end{bmatrix}D}} \\ 
       &= \frac{(D_1+D_2)'(D_1-D_2)}{\sqrt{D'R S_p R V R S_p R D}} \\ 
        &= \frac{\pi_1'\pi_2}{\sqrt{\pi' S_p\Omega S_p \pi}} 
\end{align}
where $S_p = \begin{bmatrix} 0 & I_{d_z} \\ I_{d_z} & 0 \end{bmatrix}$.




It is further useful to standardize $\pi$.  
Notice that 
\begin{align*}
 \Omega &= RVR\\
&= R\bigg((U'E[u_iu_i']U)\otimes I_{d_z}\bigg)R\\
&=\bigg(rU'E[u_iu_i']Ur\bigg)\otimes I_{d_z}\\
&= \Sigma\otimes I_{d_z}
\end{align*}
where $r = \begin{bmatrix}
1 & 1 \\ 1 & -1
\end{bmatrix}$




We partition $\Sigma$, a symmetric and positive definite 2$\times$ 2 matrix into 4 scalars:
$$
\Sigma = \begin{bmatrix}
\sigma^2_{I} & \sigma_{I,II}\\
\sigma_{I,II} & \sigma^2_{II}
\end{bmatrix}
$$
$\sigma^2_{I}$.  Let $\Psi = (\Psi_{I}',\Psi_{II}')= (\sigma_{II}^{-1} \pi_1',\sigma_{II}^{-1} \pi_2')'\sim N(\pi_0^{std}, \Omega^{std}\otimes I_{d_z} )$, where $\Psi_0 = (\Psi_{01}',\Psi_{02}')' =  (\sigma_{I}^{-1} A^{1/2}_{zz} (q_1 + q_2) ,  \sigma_{II}^{-1} A^{1/2}_{zz} (q_1 - q_2))$ and  $\Sigma^{std} = \begin{bmatrix} 1 & \rho \\ \rho & 1 \end{bmatrix}$, and  $\rho=\sigma_{I}^{-1}\sigma_{II}^{-1}\sigma_{I,II}$ is the correlation between any element of $\Psi_1$ and any element of  $\Psi_2$. Notice, with $\Sigma^{std}$ defined, we can rewrite $\Omega$ as:
\begin{align*}
    \Omega &= \Sigma \otimes I_{dz}\\
    &= \begin{bmatrix}
    \sigma_{I} I_{dz} & 0 I_{dz}\\ 0 I_{dz} & \sigma_{II} I_{dz}
    \end{bmatrix} \bigg(\Sigma^{std}\otimes I_{dz}\bigg)\begin{bmatrix}
    \sigma_{I} I_{dz} & 0 I_{dz}\\ 0 I_{dz} & \sigma_{II} I_{dz}
    \end{bmatrix}
\end{align*}
Then we can write the asymptotic distribution of the RV test statistic as a function of $\Psi$.

%\begin{align}
%    V^{std} &= \begin{bmatrix}1 & \rho\\ \rho & 1\end{bmatrix}\\
%    &= \begin{bmatrix}V_{11}^{-1/2} & 0 \\ 0 & V_{22}^{-1/2}\end{bmatrix} \begin{bmatrix}V_{11} & V_{12}\\ V_{12} & V_{22}\end{bmatrix} \begin{bmatrix}V_{11}^{-1/2} & 0 \\ 0 & V_{22}^{-1/2}\end{bmatrix}\\
%    &= S_VVS_V
%\end{align}
%so that 
%\begin{align}V &= \begin{bmatrix}V_{11}^{1/2} & 0 \\ 0 & V_{22}^{1/2}\end{bmatrix} \begin{bmatrix} 1& \rho \\ \rho & 1\end{bmatrix} \begin{bmatrix}V_{11}^{1/2} & 0 \\ 0 & V_{22}^{1/2}\end{bmatrix}\\
%&=S_V^{-1} V^{std} S_V^{-1}\end{align}

\begin{align}
     \frac{\pi_1'\pi_2}{\sqrt{\pi' S_p\Omega S_p \pi}} 
    &= \frac{\pi_1'\pi_2}{\sqrt{\pi' S_p\begin{bmatrix}
    \sigma_{I} I_{dz} & 0 I_{dz}\\ 0 I_{dz} & \sigma_{II} I_{dz}
    \end{bmatrix} \bigg(\Sigma^{std}\otimes I_{dz}\bigg)\begin{bmatrix}
    \sigma_{I} I_{dz} & 0 I_{dz}\\ 0 I_{dz} & \sigma_{II} I_{dz}
    \end{bmatrix}S_p \pi}} \\
    %&= \frac{\pi_1'\pi_2}{\sqrt{\pi' S_p S^{-1}_\Omega\Omega^{std} S^{-1}_\Omega S_p \pi}} \\
    &= \frac{\pi_1'\pi_2}{\sqrt{\begin{bmatrix}\sigma_{I} \pi_2'  &  \sigma_{II} \pi_1'  \end{bmatrix}\bigg(\Sigma^{std}\otimes I_{dz}\bigg) \begin{bmatrix}  \sigma_{I} \pi_2\\ \sigma_{II} \pi_1  \end{bmatrix}}} \\
        &=\frac{\sigma_{I}^{-1}\sigma_{II}^{-1}}{\sigma_{I}^{-1}\sigma_{II}^{-1}} \frac{\pi_1'\pi_2}{\sqrt{\begin{bmatrix}\sigma_{I} \pi_2'  &  \sigma_{II} \pi_1'  \end{bmatrix}\bigg(\Sigma^{std}\otimes I_{dz}\bigg) \begin{bmatrix}  \sigma_{I} \pi_2\\ \sigma_{II} \pi_1  \end{bmatrix}}} \\
                %&=\frac{\pi_1^{std}'\pi_2^{std}}{\sqrt{\begin{bmatrix}\Omega_{22}^{-1/2} \pi_2'  &  \Omega_{11}^{-1/2} \pi_1'  \end{bmatrix}\Omega^{std} \begin{bmatrix}  \Omega_{22}^{-1/2} \pi_2\\ \Omega_{11}^{-1/2} \pi_1  \end{bmatrix}}} \\
                &=\frac{\Psi_{I}'\Psi_{II}}{\sqrt{\begin{bmatrix}\sigma_{1}^{-1} \pi_1 \\\sigma_{II}^{-1} \pi_2    \end{bmatrix}'S_p\bigg(\Sigma^{std} \otimes I_{dz} \bigg)S_p\begin{bmatrix}  \sigma_{I}^{-1} \pi_1 \\\sigma_{II}^{-1} \pi_2 \end{bmatrix}}}\\          %&=\frac{\pi_1^{std}'\pi_2^{std}}{\sqrt{(S_\Omega\pi)'S_p\Omega^{std} S_\Omega\pi}}\\
     &=\frac{\Psi_I'\Psi_{II}}{\sqrt{\Psi'S_p\bigg(\Sigma^{std}\otimes I_{dz}\bigg) S_p\Psi}}
\end{align}
Finally,
\begin{align}
    T^{RV} \rightarrow_d \frac{\Psi_{I}'\Psi_{II}}{\sqrt{\Psi'S_p(\Sigma^{std}\otimes I_{dz}) S_p\Psi}}
\end{align}
Further notice that we can simplify the denominator given 
$$S_p(\Sigma^{std}\otimes I_{dz}) S_p = 
\begin{bmatrix}
1 & \rho\\
\rho & 1
\end{bmatrix}\otimes I_{dz} = \Sigma^{std}\otimes I_{dz}
$$ 
such that 
\begin{align}
    T^{RV} \rightarrow_d \frac{\Psi_{I}'\Psi_{II}}{\sqrt{\Psi'(\Sigma^{std}\otimes I_{dz})\Psi}}
\end{align}

%$V = \begin{bmatrix}
%\sigma^2_{\omega_0} + \sigma^2_{e_1} + 2 \sigma_{\omega_0 e_1} &\sigma^2_{\omega_0} + \sigma_{\omega_0 e_1}+ \sigma_{\omega_0 e_2} + \sigma_{e_1 e_2} \\
%\sigma^2_{\omega_0} + \sigma_{\omega_0 e_1}+ \sigma_{\omega_0 e_2} + \sigma_{e_1 e_2} & \sigma^2_{\omega_0} + \sigma^2_{e_2} + 2 \sigma_{\omega_0 e_2}
%\end{bmatrix}\otimes I_{d_z}$
%\begin{align}
%    \Omega &= RVR\\
 %   &= R \begin{bmatrix}
%\sigma^2_{\omega_0} + \sigma^2_{e_1} + 2 \sigma_{\omega_0 e_1} &\sigma^2_{\omega_0} + \sigma_{\omega_0 e_1}+ \sigma_{\omega_0 e_2} + \sigma_{e_1 e_2} \\
%\sigma^2_{\omega_0} + \sigma_{\omega_0 e_1}+ \sigma_{\omega_0 e_2} + \sigma_{e_1 e_2} & \sigma^2_{\omega_0} + \sigma^2_{e_2} + 2 \sigma_{\omega_0 e_2}
%\end{bmatrix}\otimes I_{d_z} R\\
%&=  \begin{bmatrix}
%2\sigma^2_{\omega_0} + \sigma^2_{e_1} + 3  \sigma_{\omega_0 e_1} + \sigma_{\omega_0 e_2} + \sigma_{e_1 e_2} &2\sigma^2_{\omega_0} + \sigma^2_{e_2} + \sigma_{\omega_0 e_1}+ 3\sigma_{\omega_0 e_2} + \sigma_{e_1 e_2} \\
%\sigma^2_{e_1}+ \sigma_{\omega_0 e_1}- \sigma_{\omega_0 e_2} - \sigma_{e_1 e_2} & -\sigma^2_{e_2} -  \sigma_{\omega_0 e_2} + \sigma_{\omega_0 e_1} + \sigma_{e_1e_2}
%\end{bmatrix}\otimes I_{d_z}R\\
%&=  \begin{bmatrix}
%4\sigma^2_{\omega_0} + \sigma^2_{e_1} + \sigma^2_{e_2} + 4  \sigma_{\omega_0 e_1} + 4 \sigma_{\omega_0 e_2} + 2\sigma_{e_1 e_2} &\sigma^2_{e_1} - \sigma^2_{e_2} + 2\sigma_{\omega_0 e_1}-2\sigma_{\omega_0 e_2}  \\
%\sigma^2_{e_1} - \sigma^2_{e_2} + 2\sigma_{\omega_0 e_1}-2\sigma_{\omega_0 e_2}& \sigma^2_{e_1} +  \sigma^2_{e_2} - 2 \sigma_{e_1e_2}
%\end{bmatrix}\otimes I_{d_z}
%\end{align}
Notice that the asymptotic distribution of the  RV test statistic depends on three paramaters, $\Psi_{01}, \Psi_{02}$, and $\rho$. The null space in this parameterization is characterized by $\Psi_{01}'\Psi_{02} = 0$.  In the null space, but far from the origin, instruments are relatively strong and the RV test statistic converges to a standard normal.  However, close to the origin, the RV test suffers from a size distortion due to degeneracy.   



\subsection{Deriving the Critical Values}

Using this asymptotic distribution we find thresholds for concentration parameters according to the procedure in Stock and Yogo (2005), which finds critical values for the first stage F-statistic which ensure that inference is reliable. In particular, we are looking for values of $\pi_0^* = (\pi^*_{01},\pi^*_{02})$ in the null space such that:
\begin{align}\label{eq:iota_star}
    \Pr[\mid T^{RV}\mid>1.96 \mid \pi_0 =\pi_0^*] = r,
\end{align}
where $r>\alpha$ is the worst case size exceeding the nominal size of the test.  For a given choice of $r$, we can find $\pi_0^*$ via numerical inversion of Equation (\ref{eq:iota_star}) which involves simulating the probability using the asymptotic distribution of $T^{RV}$ under weak instruments derived above. 

The distribution of the RV statistic depends on $\rho$.  For each guess of $\pi^*_0$, we evaluate the probability over a fine grid of $\rho$ from -1 to 1 by steps of 0.05.  To obtain conservative thresholds, we focus on the worst case size across $\rho$'s. Thus, instead of inverting Equation (\ref{eq:iota_star}), we invert the following:
$$P(\pi_0^*) = \min_\rho \Pr[\mid T^{RV} > 1.96\mid \pi_0 = \pi_0^*, \rho] = r$$




 When $d_z = 1$, we can search directly over values of $\pi_0$.  However, when $d_z>1$, the vector $\pi_0$ has dimension $2 d_z,$ so that solving equation (\ref{eq:iota_star}) potentially involves a high-dimensional search. In this case, we find that the sum of the concentration parameters that determine instrument strength, given by $\mu_{1} = \pi_{01}'\pi_{01}$ and  $\mu_2 = \pi_{02}'\pi_{02}$ characterizes well the size of the test.  To establish this fact, we search over a grid of $(\mu_1,\mu_2)$.  For each pair, we search over multiple values of $\pi_0$  which rationalize these concentration parameters and a fine grid of $\rho$ values.  We perform this exercise for two to fifteen instruments.  In Figure \ref{fig:size_SY} we show a contour plot of the size of the test in the space of $(\mu_1,\mu_2)$ for 15 instruments, which is representative of all our simulations.  As maximal size depends on the sum of $\mu_1$ and $\mu_2$, we can solve for $\pi^*_0$ by finding the corresponding value of the sum of $\mu_1$ and $\mu_2$ denoted $\mu^*$.  
 \begin{figure}[ht]
     \centering
      \caption{Relationship Between Maximal Size and Concentration Parameters}
     \includegraphics[scale = 0.6]{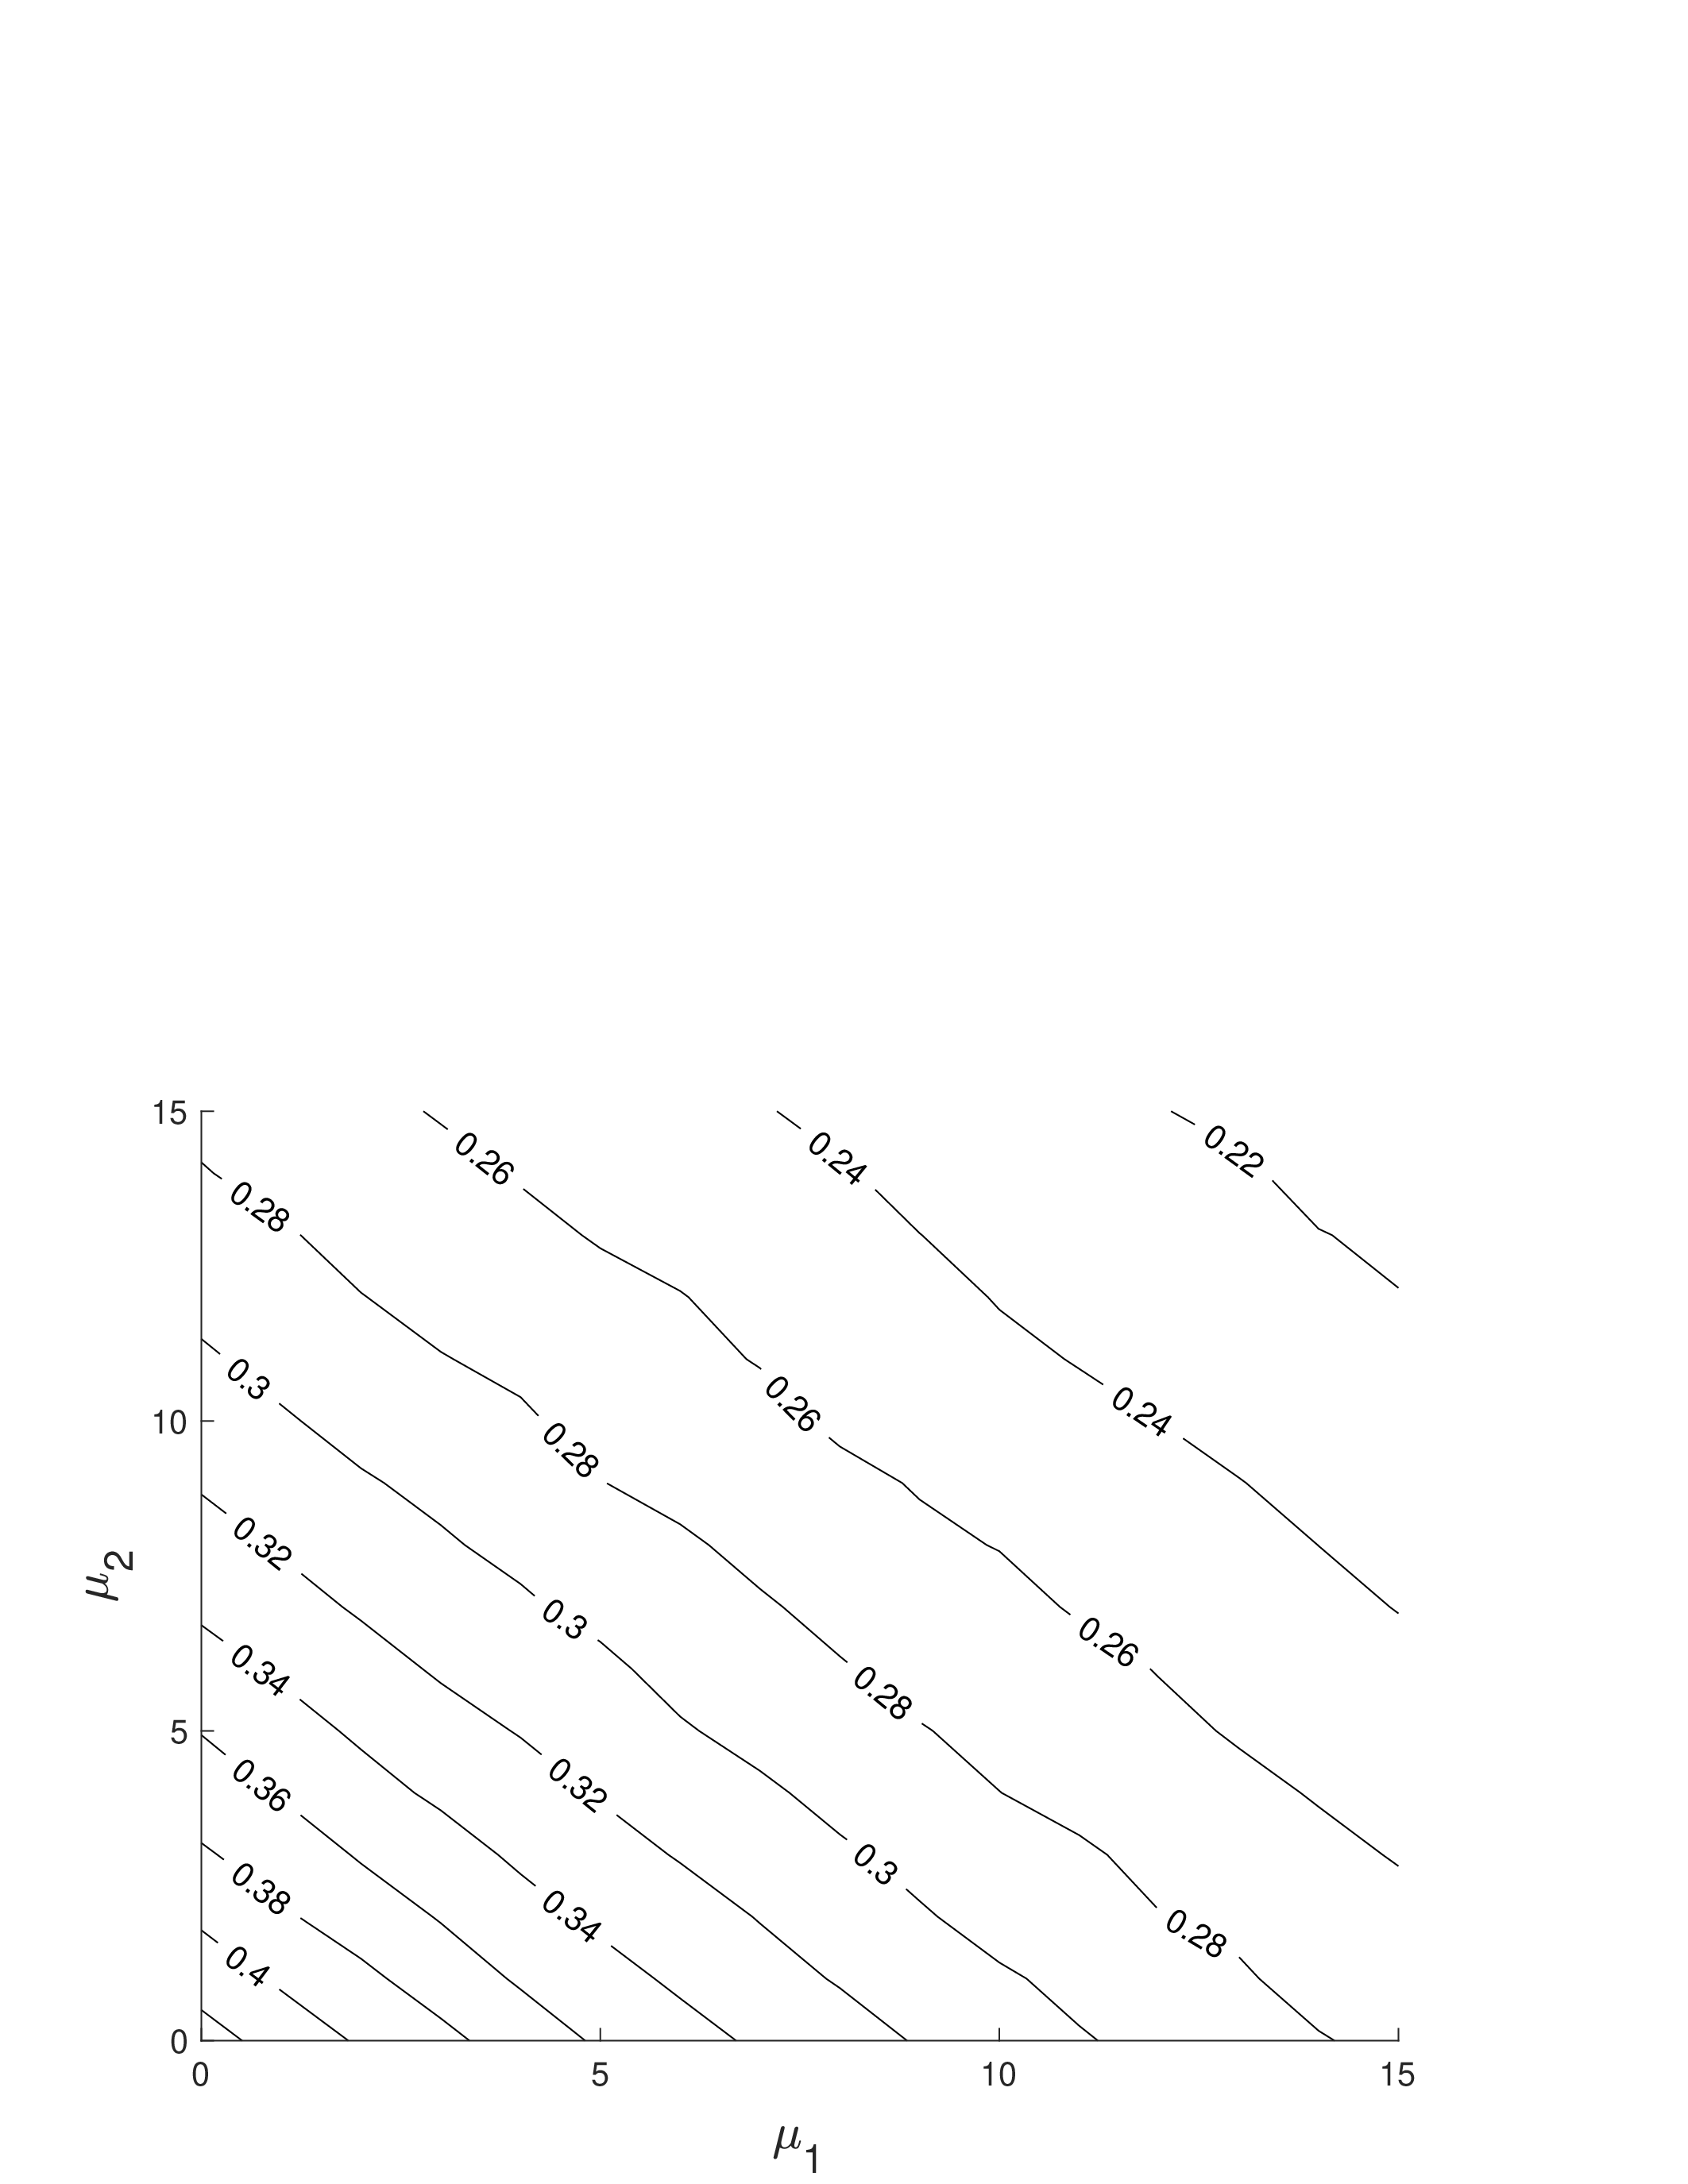}
    \label{fig:size_SY}
    \caption*{\footnotesize{This figure illustrates in the space of concentration parameters $\mu_1$ and $\mu_2$ contour lines for maximal size for $d_z=15$.}}
\end{figure}


  


While we cannot estimate $\mu_1$ and $\mu_2$ in the data, it is possible to test the hypothesis that $\mu_1+\mu_2 > \mu^*$.  Specifically, we can compute F-statistics for two regressions (i) $2p-\Delta_1-\Delta_2$  on instruments and (ii) $\Delta_1-\Delta_2$ on instruments as follows, letting the residuals from these regressions be $\hat\zeta_1$ and $\hat\zeta_2$ respectively. 
\begin{align*}
    F_1 &= \frac{((z'z)^{-1}z'(2\Delta_0+2\omega_0-\Delta_1-\Delta_2))'z'z((z'z)^{-1}z'(z(2\Delta_0+2\omega_0-\Delta_1-\Delta_2))}{d_z\hat\sigma^2_{\zeta_1}},\\
&=    \frac{((z'z)^{-1}z'(z\frac{q_1+q_2}{\sqrt{n}}+\zeta_1))'z'z((z'z)^{-1}z'(z\frac{q_1+q_2}{\sqrt{n}}+\zeta_1))}{d_z\hat\sigma^2_{\zeta_1}},\\
&= \frac{ ( \hat A_{zz}^{1/2}(q_1+q_2)\hat A_{zz}^{-1/2}\frac{z'\zeta_1}{\sqrt{n}})'( \hat A_{zz}^{1/2}(q_1+q_2)+\hat A_{zz}^{-1/2}\frac{z'\zeta_1}{\sqrt{n}})}{d_z\hat\sigma^2_{\zeta_1}},\\
&= \frac{( \hat A_{zz}^{1/2}(q_1+q_2)+\hat A_{zz}^{-1/2}\frac{z'\zeta_1}{\sqrt{n}})'}{\sqrt{d_z}\hat\sigma_{\zeta_1}}\frac{( \hat A_{zz}^{1/2}(q_1+q_2)+\hat A_{zz}^{-1/2}\frac{z'\zeta_1}{\sqrt{n}})}{\sqrt{d_z}\hat\sigma_{\zeta_1}},\\
 d_z F_1&\rightarrow_d \chi^2_{d_z}(\pi_{01}'\pi_{01})
\end{align*}
where $\zeta_1=2\omega_0 + e_1 + e_2$ and $\sigma^2_{\zeta_1} = 4\sigma^2_{\omega_0} + \sigma^2_{e_1} + \sigma^2_{e_2} + 4\sigma_{\omega_0 e_1} + 4\sigma_{\omega_0 e_2} + 2\sigma_{e_1 e_2}=\Omega_{11}$.

Also, 
\begin{align*}
    F_2 &= \frac{(\hat\Gamma_1-\hat\Gamma_2)'z'z(\hat\Gamma_1-\hat\Gamma_2)}{d_z\hat\sigma^2_{\zeta_2}},\\
&=    \frac{((z'z)^{-1}z'(\Delta_1-\Delta_2))'z'z((z'z)^{-1}z'(\Delta_1-\Delta_2)}{d_z\hat\sigma^2_{\zeta_2}},\\
&=    \frac{((z'z)^{-1}z'(z\frac{q_1-q_2}{\sqrt{n}}+\zeta_2))'z'z((z'z)^{-1}z'(z\frac{q_1-q_2}{\sqrt{n}}+\zeta_2))}{d_z\hat\sigma^2_{\zeta_2}},\\
&= \frac{ ( \hat A_{zz}^{1/2}(q_1-q_2)+\hat A_{zz}^{-1/2}\frac{z'\zeta_2}{\sqrt{n}})'( \hat A_{zz}^{1/2}(q_1-q_2)+\hat A_{zz}^{-1/2}\frac{z'\zeta_2}{\sqrt{n}})}{d_z\hat\sigma^2_{\zeta_2}},\\
&= \frac{( \hat A_{zz}^{1/2}(q_1-q_2)+\hat A_{zz}^{-1/2}\frac{z'\zeta_2}{\sqrt{n}})'}{\sqrt{d_z}\hat\sigma_{\zeta_2}}\frac{( \hat A_{zz}^{1/2}(q_1-q_2)+\hat A_{zz}^{-1/2}\frac{z'\zeta_2}{\sqrt{n}})}{\sqrt{d_z}\hat\sigma_{\zeta_2}},\\
 d_z F_2&\rightarrow_d \chi^2_{d_z}(\pi_{02}'\pi_{02})
\end{align*}

 We can find a critical value ${cv}$ and corresponding to a test of the null that  $\mu_1+\mu_2 = \mu^*$ that has nominal size 0.05.
 Under the assumption that $F_1$ and $F_2$ are independent, we can write:
\begin{align*}
\Pr[F_1+F_2 \geq {cv} \mid \mu = {\mu}^*]&=    \Pr[d_z (F_1+F_2) \geq d_z {cv} \mid \mu = {\mu}^*]\\ 
    &\rightarrow_p \Pr[\chi_{2d_z}^2({\mu}^*) \geq d_z {cv} ]\\
    &=1-G\bigg( d_z {cv},{\mu}^*\bigg)\\
    &= 0.05
\end{align*}
where $G$ is the cdf of a non-central $\chi_{2d_z}^2$ distribution. So, we can invert to get the critical value as:
$${cv} = \frac{1}{d_z}G^{-1}(0.95,{\mu}^*).$$


  As the values of $\mu^*$ and therefore the critical values depend on $r$ and $d_z$, we report in Table \ref{tab:Tab_StockYogo} critical values for $r = 0.10$, 0.15, 0.20 and 0.25, and for $dz \in [1,30]$. 
