# Supplementary material for: Testing Firm Conduct
Source: arXiv:2301.06720 source file (2024-01-17)
Supplement: Supplementary file 30 [file BCS_Appendix.tex]

\subsection{Choosing the Weight Matrix}\label{sec:weightmatrix}

 The RV test statistic described in Section \ref{sec:thetests} depends on a weight matrix $W$ and \cite{hp11} show that the RV test is sensitive to this choice.\footnote{Cox, EB, and AR also depend on weighting. The plims of EB and Cox also depend on Euclidean distance when $W = (\frac{z'z}{n})^{-1}$}   While we adopt $W = (\frac{z'z}{n})^{-1}$ throughout,  Proposition  \ref{prop:plims_TE2} can be modified for a generic $W$ as: 
\begin{align*}
\frac{T^{RV}}{\sqrt{n}}&\rightarrow_p \frac{E[(\Delta^z_{1i}-\Delta^z_{0i})z_iWz_i(\Delta^z_{1i}-\Delta^z_{0i})] - E[(\Delta^z_{2i}-\Delta^z_{0i})z_iWz_i(\Delta^z_{2i}-\Delta^z_{0i})]}{\sigma_{RV}}.
\end{align*}
The RV test asymptotically rejects in favor of the model whose predicted markups are closer to the true predicted markups based on a distance measure defined by $W$.     

In general, we feel $W = (\frac{z'z}{n})^{-1}$ is preferable to any alternative choice. When $W = (\frac{z'z}{n})^{-1}$, the RV numerator is measured via the Euclidean distance which permits intuitive comparisons of models.  This distance metric also directly implements the testability condition in \cite{bh14} as shown in  Lemma \ref{lemma1}.      Furthermore, the efficiency concerns in support of the optimal weight matrix do not extend to testing.\looseness=-1 


Choosing $W$ different from  $(\frac{z'z}{n})^{-1}$  may also increase the scope of degeneracy. Consider the weight matrix  
$\widetilde W = (\hat\Gamma_1-\hat\Gamma_2)(\hat\Gamma_1-\hat\Gamma_2)'$.  If instruments are chosen flexibly as discussed in Section  \ref{sec:sieveIJIVE}, $\widetilde W$ can be used to construct the version of the RV test in \cite{bcs20}:
%\begin{align*}
%    \widetilde T^{RV} &= \frac{\sqrt{n}(g_1\widetilde W g_1 - g_2 \widetilde W g_2)}{\hat{ \tilde{ \sigma}}}\\
%    &= \frac{\sqrt{n}((\tilde \Delta_1 - \tilde \Delta_2)'\omega_1)^2 - (\tilde \Delta_1 - \tilde \Delta_2)'\omega_2)^2)}{n \hat{ \tilde{ \sigma}}}.
%\end{align*}
\begin{align*}
    \widetilde T^{RV} = \frac{\sqrt{n}(g_1\widetilde W g_1 - g_2 \widetilde W g_2)}{\hat{ \tilde{ \sigma}}}
    = \frac{\sqrt{n}((\tilde \Delta_1 - \tilde \Delta_2)'\omega_1)^2 - (\tilde \Delta_1 - \tilde \Delta_2)'\omega_2)^2)}{n \hat{ \tilde{ \sigma}}}.
\end{align*}

In Appendix \ref{sect:bcs_app}, we show how  $\widetilde T^{RV}$ relates to $T^{RV}$ defined with $W=(\frac{z'z}{n})^{-1}$. As long as $\widetilde T^{RV}$ is not degenerate, the two test statistics are identical, and thus asymptotically rely on the comparison of Euclidean distances in predicted markups. However, $\widetilde T^{RV}$ may be degenerate when $T^{RV}$ is not. From Proposition \ref{prop:degen}, $T^{RV}$
is degenerate when $\hat \Gamma_1$, $\hat \Gamma_2$, \textit{and} $\hat \Gamma_0$ approach each other. Instead, whenever $\hat \Gamma_1$ and $\hat \Gamma_2$ approach each other, $\widetilde W$ approaches the zero matrix and  $\widetilde T^{RV}$ is degenerate.
 
 \begin{figure}[h!]
     \centering
      \caption{Weight Matrix and Degeneracy}
     \input{Graphs/GammaSpace}
    \label{fig:gamma_space_deg}
    \caption*{\footnotesize{This figure illustrates (i) the null space of the RV test (both 45-degree lines), (ii) the region of degeneracy for $\widetilde T^{RV}$ (the red 45-degree line), and (iii) the region of degeneracy for $T^{RV}$ (the origin).}} \vspace{-0.5cm}
\end{figure}

While the discussion in Appendix \ref{sect:bcs_app} holds in general, we can visually compare the region of degeneracy for $T^{RV}$ and $\widetilde T^{RV}$  when one instrument is used for testing. Since $\Gamma_m$ is a scalar, in Figure \ref{fig:gamma_space_deg} we plot the coordinate space $(\Gamma_0 - \Gamma_1,\Gamma_0 - \Gamma_2)$. The null of RV corresponds to both 45-degree lines. Degeneracy of $\widetilde T^{RV}$ occurs along the positive 45-degree red dashed line, whereas degeneracy of $T^{RV}$ only occurs at the origin. In practice, expanding the region of degeneracy may be consequential. Consider a situation where the two models approach each other, but are far from the truth because of misspecification in demand or cost. In this case, $\widetilde T^{RV}$ is degenerate (with problematic consequences for the size and power of the test) but $T^{RV}$ is not.  Furthermore, our diagnostic for weak instruments for testing is only valid with the weight matrix $W=(\frac{z'z}{n})^{-1}$, so one cannot use the critical values in Table \ref{tab:Tab_StockYogo} to diagnose degeneracy of $\widetilde T^{RV}$.\looseness=-1   








Using a sieve expansion (see Section \ref{sec:sieveIJIVE}), we can write sample predicted markups for model $m$ as: $$\hat{\tilde{\Delta}}_m = z\hat\Gamma_m.$$
 Then we can write the sample difference in predicted markups for models 1 and 2 as :
\begin{align}
    \widehat{D\Delta}_{12} &= \hat{\tilde{\Delta}}_1 - \hat{\tilde{\Delta}}_2\label{eq:pred_diff1}\\ &= z(z'z)^{-1}z'(\Delta_1-\Delta_2)\\
    &= z(\hat\Gamma_1-\hat\Gamma_2).\label{eq:pred_diff}
\end{align}

\noindent Now we consider $Q^{BCS}_m$ as defined in \cite{bcs20}.\footnote{Note that in \cite{bcs20} they use a random forest to obtain (\ref{eq:pred_diff1}). In large samples, both sieve and random forests should well approximate the true differences in predicted markups.}
\begin{align}
    Q^{BCS}_m &= (n^{-1}\sum_i \omega_{mi}\widehat{D\Delta}_{12i})^2\\
    &=\bigg(\frac{\widehat{D\Delta}_{12}'\omega_m}{n}\bigg)^2\\
    &=\bigg(\frac{\widehat{D\Delta}_{12}'\omega_m}{n}\bigg)'\bigg(\frac{\widehat{D\Delta}_{12}'\omega_m}{n}\bigg) 
\end{align}

\noindent Plugging in (\ref{eq:pred_diff}), we get
\begin{align}
    Q^{BCS}_m &= \bigg(\frac{(\hat\Gamma_1-\hat\Gamma_2)'z'\omega_m}{n}\bigg)'\bigg(\frac{(\hat\Gamma_1-\hat\Gamma_2)'z'\omega_m}{n}\bigg) \\
    &= \frac{\omega_m'z}{n}(\hat\Gamma_1-\hat\Gamma_2)(\hat\Gamma_1-\hat\Gamma_2)'\frac{z'\omega_m}{n}
\end{align}
Let $g_m = \frac{z'\omega_m}{n}$. 
Then we have 
\begin{align}
    Q^{BCS}_m&= g_m'(\hat\Gamma_1-\hat\Gamma_2)(\hat\Gamma_1-\hat\Gamma_2)'g_m.
\end{align}
So, $Q^{BCS}_m$ can be written as the GMM objective function constructed using orthogonality moments for model $m$ with weight matrix $\widetilde W = (\hat\Gamma_1-\hat\Gamma_2)(\hat\Gamma_1-\hat\Gamma_2)'$.  We can rewrite $\widetilde W$ as:
\begin{align}
    \widetilde W &=(\hat\Gamma_1-\hat\Gamma_2)(\hat\Gamma_1-\hat\Gamma_2)'\\
    &= (z'z)^{-1}z'(\Delta_1-\Delta_2)(\Delta_1-\Delta_2)'z(z'z)^{-1}\\
    &= (\frac{z'z}{n})^{-1}\frac{z'(\Delta_1-\Delta_2)}{n}\frac{(\Delta_1-\Delta_2)'z}{n}(\frac{z'z}{n})^{-1}\\
    &= W\frac{z'(\Delta_1-\Delta_2)}{n}\frac{(\Delta_1-\Delta_2)'z}{n}W
\end{align}
where $W = (\frac{z'z}{n})^{-1}$.

\noindent  Now we show the relationship between $Q^{BCS}_1 - Q^{BCS}_2$ and $Q_1-Q_2$: 
\begin{align}
    Q^{BCS}_1-Q^{BCS}_2 
    %&= g_1' \widetilde W g_1 - g_2' \widetilde W g_2\\
    &= (g_1 - g_2)' \widetilde W (g_1 + g_2)\\
     &= (g_1 - g_2)' W\frac{z'(\Delta_1-\Delta_2)}{n}\frac{(\Delta_1-\Delta_2)'z}{n}W (g_1 + g_2)\\
     &= (g_1 - g_2)' W\frac{z'(\Delta_1-\Delta_2)}{n}\frac{(-p + \Delta_1 + p-\Delta_2)'z}{n}W (g_1 + g_2)\\
%     &= (g_1 - g_2)' W\frac{z'(\Delta_1-\Delta_2)}{n}\frac{(-\omega_1 +\omega_2)'z}{n}W (g_1 + g_2)\\
          &= -(g_1 - g_2)' W\frac{z'(\Delta_1-\Delta_2)}{n}(g_1-g_2)W (g_1 + g_2)\\
                    &= -(g_1 - g_2)' W\frac{z'(\Delta_1-\Delta_2)}{n}\bigg(g_1'Wg_1 -g_2'Wg_2\bigg)\\
 %       &= -\frac{(\omega_1 - \omega_2)'z}{n} W\frac{z'(\Delta_1-\Delta_2)}{n}(Q_1 - Q_2)\\
        &= -\frac{(p-\Delta_1 - p+\Delta_2)'z}{n} W\frac{z'(\Delta_1-\Delta_2)}{n}(Q_1 - Q_2)\\
         &= \frac{(\Delta_1 -\Delta_2)'z}{n} W\frac{z'(\Delta_1-\Delta_2)}{n}(Q_1 - Q_2)
        %
       % &= (z'(\omega_1 - \omega_2))' (\hat\Gamma_1 - \hat\Gamma_2)(\hat\Gamma_1 - \hat\Gamma_2)'(z'(\omega_1 + \omega_2))\\
        %&= (z'(p-\Delta_1 - p+ \Delta_2))' (\hat\Gamma_1 - \hat\Gamma_2)(\hat\Gamma_1 - \hat\Gamma_2)'(z'(p-\Delta_1 + p- \Delta_2))\\
        %&= (z'( \Delta_2-\Delta_1 ))' (\hat\Gamma_1 - \hat\Gamma_2)(\hat\Gamma_1 - \hat\Gamma_2)'(z'(2p-\Delta_1 - \Delta_2))\\
         %       &= (z'( \Delta_2-\Delta_1 ))' W\frac{z'(\Delta_1-\Delta_2)}{n}\frac{(\Delta_1-\Delta_2)'z}{n}W(z'(2p-\Delta_1 - \Delta_2))\\
          %  &= (z'( \Delta_1-\Delta_2 ))' W\frac{z'(\Delta_1-\Delta_2)}{n}\frac{(\Delta_2-\Delta_1)'z}{n}W(z'(2p-\Delta_1 - \Delta_2))\\
           %  &= (z'( \Delta_1-\Delta_2 ))' W\frac{z'(\Delta_1-\Delta_2)}{n}(Q_1-Q_2)\\
            %   &= \frac{( \Delta_1-\Delta_2 )'z}{n} W\frac{z'(\Delta_1-\Delta_2)}{n}(Q_1-Q_2)\\
             %  &= \frac{( \Delta_1-\Delta_2 )'z}{n} WW^{-1}W\frac{z'(\Delta_1-\Delta_2)}{n}(Q_1-Q_2)\\
              % &= \frac{( \Delta_1-\Delta_2 )'z}{n} (\frac{z'z}{n})^{-1}(\frac{z'z}{n})(\frac{z'z}{n})^{-1}\frac{z'(\Delta_1-\Delta_2)}{n}(Q_1-Q_2)\\
               %&= \frac{( \tilde\Delta_1-\tilde\Delta_2 )'( \tilde\Delta_1-\tilde\Delta_2 )}{n} (Q_1-Q_2)\\
\end{align}
Then we can derive the following convergence in probability result  
\begin{align*}
    \frac{( \Delta_1-\Delta_2 )'z}{n} W\frac{z'(\Delta_1-\Delta_2)}{n} &\rightarrow_p (\theta_1-\theta_2)'E[\Delta_i z_i']E[z_iz_i']^{-1}E[z_i\Delta_i'](\theta_1-\theta_2)\\
    %&\rightarrow_p (\theta_1-\theta_2)'A_{z\Delta}'A_{zz}^{-1} A_{z\Delta}(\theta_1-\theta_2)\\
    &= (\Gamma_1 - \Gamma_2)'E[z_iz_i'](\Gamma_1 - \Gamma_2)\\
    &=\phi.
    \end{align*}
First suppose that the term $\phi$ is a non-zero constant, and $\sqrt{n}(Q_1-Q_2) \rightarrow_d \eta$ where $\eta$ is a generic random variable with finite second moment.  An estimate of the asymptotic variance of $\sqrt{n}( Q^{BCS}_1 - Q^{BCS}_2)$ is  $\hat\phi^2 \widehat{var}(\eta)$.  So, using this asymptotic approximation to form the RV test statistic yields:
\begin{align}
    T^{RV} &=\sqrt{n}\frac{(Q^{BCS}_1-Q^{BCS}_2)}{\hat\phi (\widehat{var}(\eta))^{1/2}}\\
    &=\sqrt{n}\frac{\hat\phi (Q_1-Q_2)}{\hat\phi (\widehat{var}(\eta))^{1/2}}\\
    &=\sqrt{n}\frac{ (Q_1-Q_2)}{ \hat\sigma^{RV}}
\end{align}
which is the test statistic we define in Section 4 of the paper. 

Instead, suppose that $\phi=0$, which occurs iff $\Gamma_1 = \Gamma_2$. In this case, the asymptotic variance of $\sqrt{n}(Q^{BCS}_1-Q^{BCS}_2 )$ is zero, and degeneracy arises. This can occur in settings where $T^{RV}$ is not degenerate. As shown in Proposition \ref{prop:degen}, the condition for $T^{RV}$ to be degenerate is that $\Gamma_1 = \Gamma_2 =\Gamma_0,$ which is a special case of degeneracy in the \cite{bcs20} version of the test statistic.
