# Supplementary material for: Testing Firm Conduct
Source: arXiv:2301.06720 source file (2024-01-17)
Supplement: Supplementary file 32 [file ManyInstruments.tex]

\subsection{Many Instruments for Testing: Bias of RV}\label{sec:manyinstr} 

The RV test fundamentally depends on predicting markups from the instruments.  When the first stage is viewed in this light, one may consider adding a large number of instruments in order to improve the predictions.  In light of Proposition \ref{prop:degen}, there may be benefits to doing so in the context of RV.  However, this comes at a cost.  The econometrics literature has discussed the problem of many instruments in an estimation context.  Specifically  \cite{b94} and \cite{cs05} show that the 2SLS estimator is inconsistent under a many instruments asymptotic.  More troubling, this asymptotic has been found to approximate well the finite sample distribution of the estimator, thus revealing substantial bias towards the OLS estimator.  The intuition, discussed in \cite{ad09} is that increasing the number of instruments overfits the endogenous variable.  In the extreme, one predicts the endogenous variable perfectly and thus reverts to OLS in the second stage.  

We show that the use of many instruments has a similar impact on the RV test that it does in 2SLS.  We first establish the analogue of OLS in testing.  Consider alternative moments
$g^{OLS}_m = \frac{\Delta'\hat\omega_m}{n}$,
which are the moments one would use to estimate Equation (\ref{eq:test}) by OLS. We define a measure of fit using these moments as $Q_m^{OLS} = g^{OLS\prime}_m(\frac{\Delta'\Delta}{n})^{-1} g^{OLS}_m$. Now we can define a version of the RV test statistic with the OLS moments: $T^{OLS} = \frac{\sqrt{n}}{\hat  \sigma_{RSS}} (Q_1^{OLS} - Q_2^{OLS}).$
As shown in Appendix XX, this test is inconsistent and has a plim given by:
$$\frac{T^{OLS}}{\sqrt{n}} &\rightarrow_p  \frac{E[(\Delta^{OLS}_i -\Delta_{1i})^2 - (\Delta^{OLS}_i -\Delta_{2i})^2]	}{\sigma_{OLS}}$$
This shows that OLS-based tests asymptotically reject in favor of the model for which the implied markups are closer to the OLS markups. Since $\Delta$ is generally correlated with $\omega$, $\Delta^{OLS}$ may be very far from $\Delta_0$.  While $T^{OLS}$ may seem artificial, we show in Appendix XX that it is equivalent to an implementation of the RV test based on residual sum of squares (RSS) which has been popular in the applied IO literature.\footnote{For example, \cite{b87}, \cite{glv92}, \cite{bd10} and \cite{bdvk13} use RSS-based procedures to test hypotheses on conduct.} 



Now, to formalize the bias of many instruments, 
we consider a many instrument asymptotic, following \cite{b94} and \cite{cs05}.   Specifically, letting $\Gamma = [\Gamma_1, \Gamma_2]$, we assume the following:

\begin{assumption}\label{as:manyinstr} Let the number of instruments grow at rate $n$ so that $\frac{d_z}{n} \rightarrow_p \delta_z > 0$.  Moreover, suppose:
(i) $\frac{\hat\Gamma'z'z\hat\Gamma}{n}\rightarrow H_1 + o_p(1)$ and (ii) $\frac{\hat\Gamma'z'z\hat\Gamma_0}{n}\rightarrow H_2 + o_p(1)$ for some matrices $H_1,H_2>0$.
\end{assumption}
The above assumption maintains that  the concentration parameters $\frac{\Gamma'z'z\Gamma}{n}$ and $\frac{\Gamma'z'z\Gamma_0}{n}$ are non-diverging as the number of instruments grows.  Thus, the variance of the predicted markups remains finite. One way to interpret this assumption is that additional instruments are eventually uninformative in predicting markups. Regardless of the interpretation, the econometrics literature has found that the asymptotic distribution obtained with this assumption is a good approximation of the finite sample performance even if $d_z$ is small (see \cite{b94} and \cite{ak95}).\looseness=-1


Under Assumption \ref{as:manyinstr}, we can characterize the behavior of the RV test statistic in a many instrument setting.  Specifically, we derive the following result:
\begin{proposition}\label{prop:biasmany} Suppose that Assumptions \ref{as:momcond}, \ref{as:regcond}, and \ref{as:manyinstr} are satisfied. Then:
\begin{align*}
    \frac{T^{RV}}{\sqrt{n}} \rightarrow_p 
    & \frac{1-\delta_z}{\sigma_{RV}}
    \bigg(E[(\Delta^z_{1i}-\Delta^z_{0i})^2] - E[(\Delta^z_{2i}-\Delta^z_{0i})^2]\bigg)
    \\&\qquad +\frac{\delta_z}{\sigma_{RV}}\bigg(E[(\Delta_{1i}-\Delta^{OLS}_i)^2] - E[(\Delta_{2i}-\Delta^{OLS}_i)^2]\bigg)
\end{align*}

\end{proposition}

Proposition \ref{prop:biasmany} sheds light on important aspects of testing with many instruments. In estimation, the presence of many instruments biases 2SLS estimates to their OLS counterpart.  Likewise, we see that the RV test is biased towards the RSS test discussed in Section \ref{sec:RSS}, which forms the moments with the endogenous markups.  The extent of the bias depends on the magnitude of $\delta_z$.  \cite{h20} states that although there is no set rule of thumb, many instruments are a serious concern whenever the number of instruments exceeds 5\% of the sample size. However, many instruments can still create significant bias below that threshold.  In fact, \cite{ak95} find severe bias in a setting where  $\frac{d_z}{n}$ is as small as 0.005.  


Thus, a researcher should be concerned when using many instruments \textit{even if they are valid}.  While valid instruments implement the condition in Lemma 1, there is no guarantee that using them to form the RV test will allow one to  achieving correct inference either in finite sample or asymptotically.  We return to the problem of many instruments in Section \ref{sec:sieveIJIVE} and propose a modification of the RV test statistic which removes the finite sample bias that they cause.
